# Supplementary material for: Physics-aware Differentiable Discrete Codesign for Diffractive Optical Neural Networks
Source: arXiv:2209.14252 source file (2022-09-28)
Supplement: Supplementary file 1 [file sec-appendix.tex]

\section{Appendix}

\subsection{Code}

Code is submitted in supplementary materials.

\subsection{Supplementary materials}

\begin{figure}[h]
    \centering
    \begin{subfigure}[b]{1\linewidth}
    \centering
        {\includegraphics[width=0.18\linewidth]{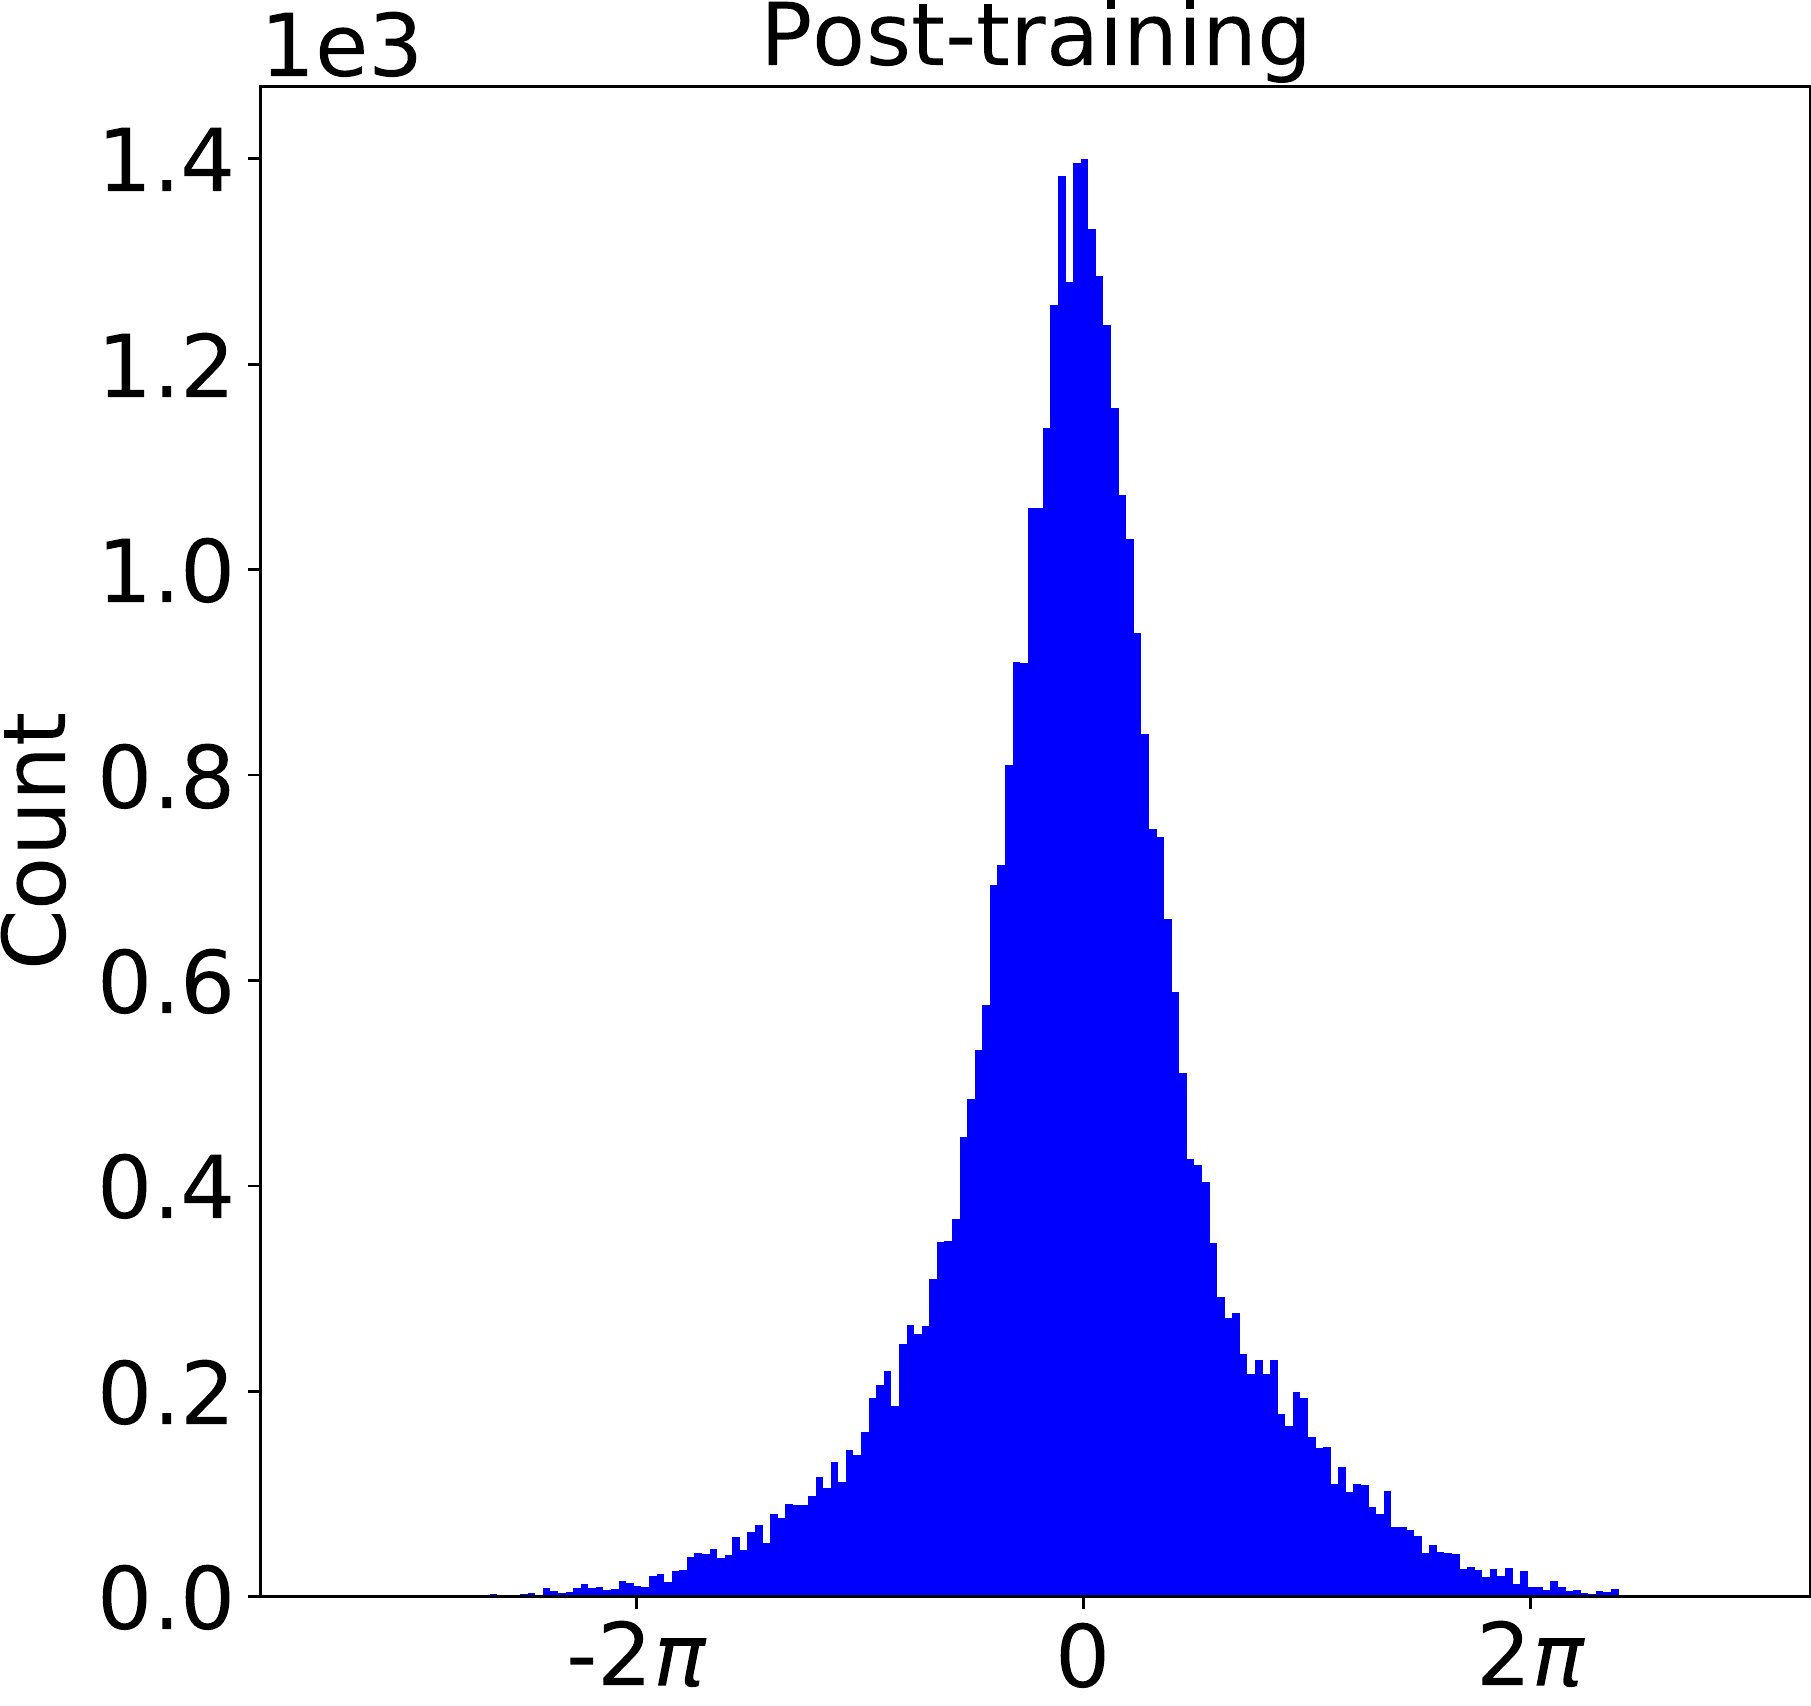}}
        {\includegraphics[width=0.18\linewidth]{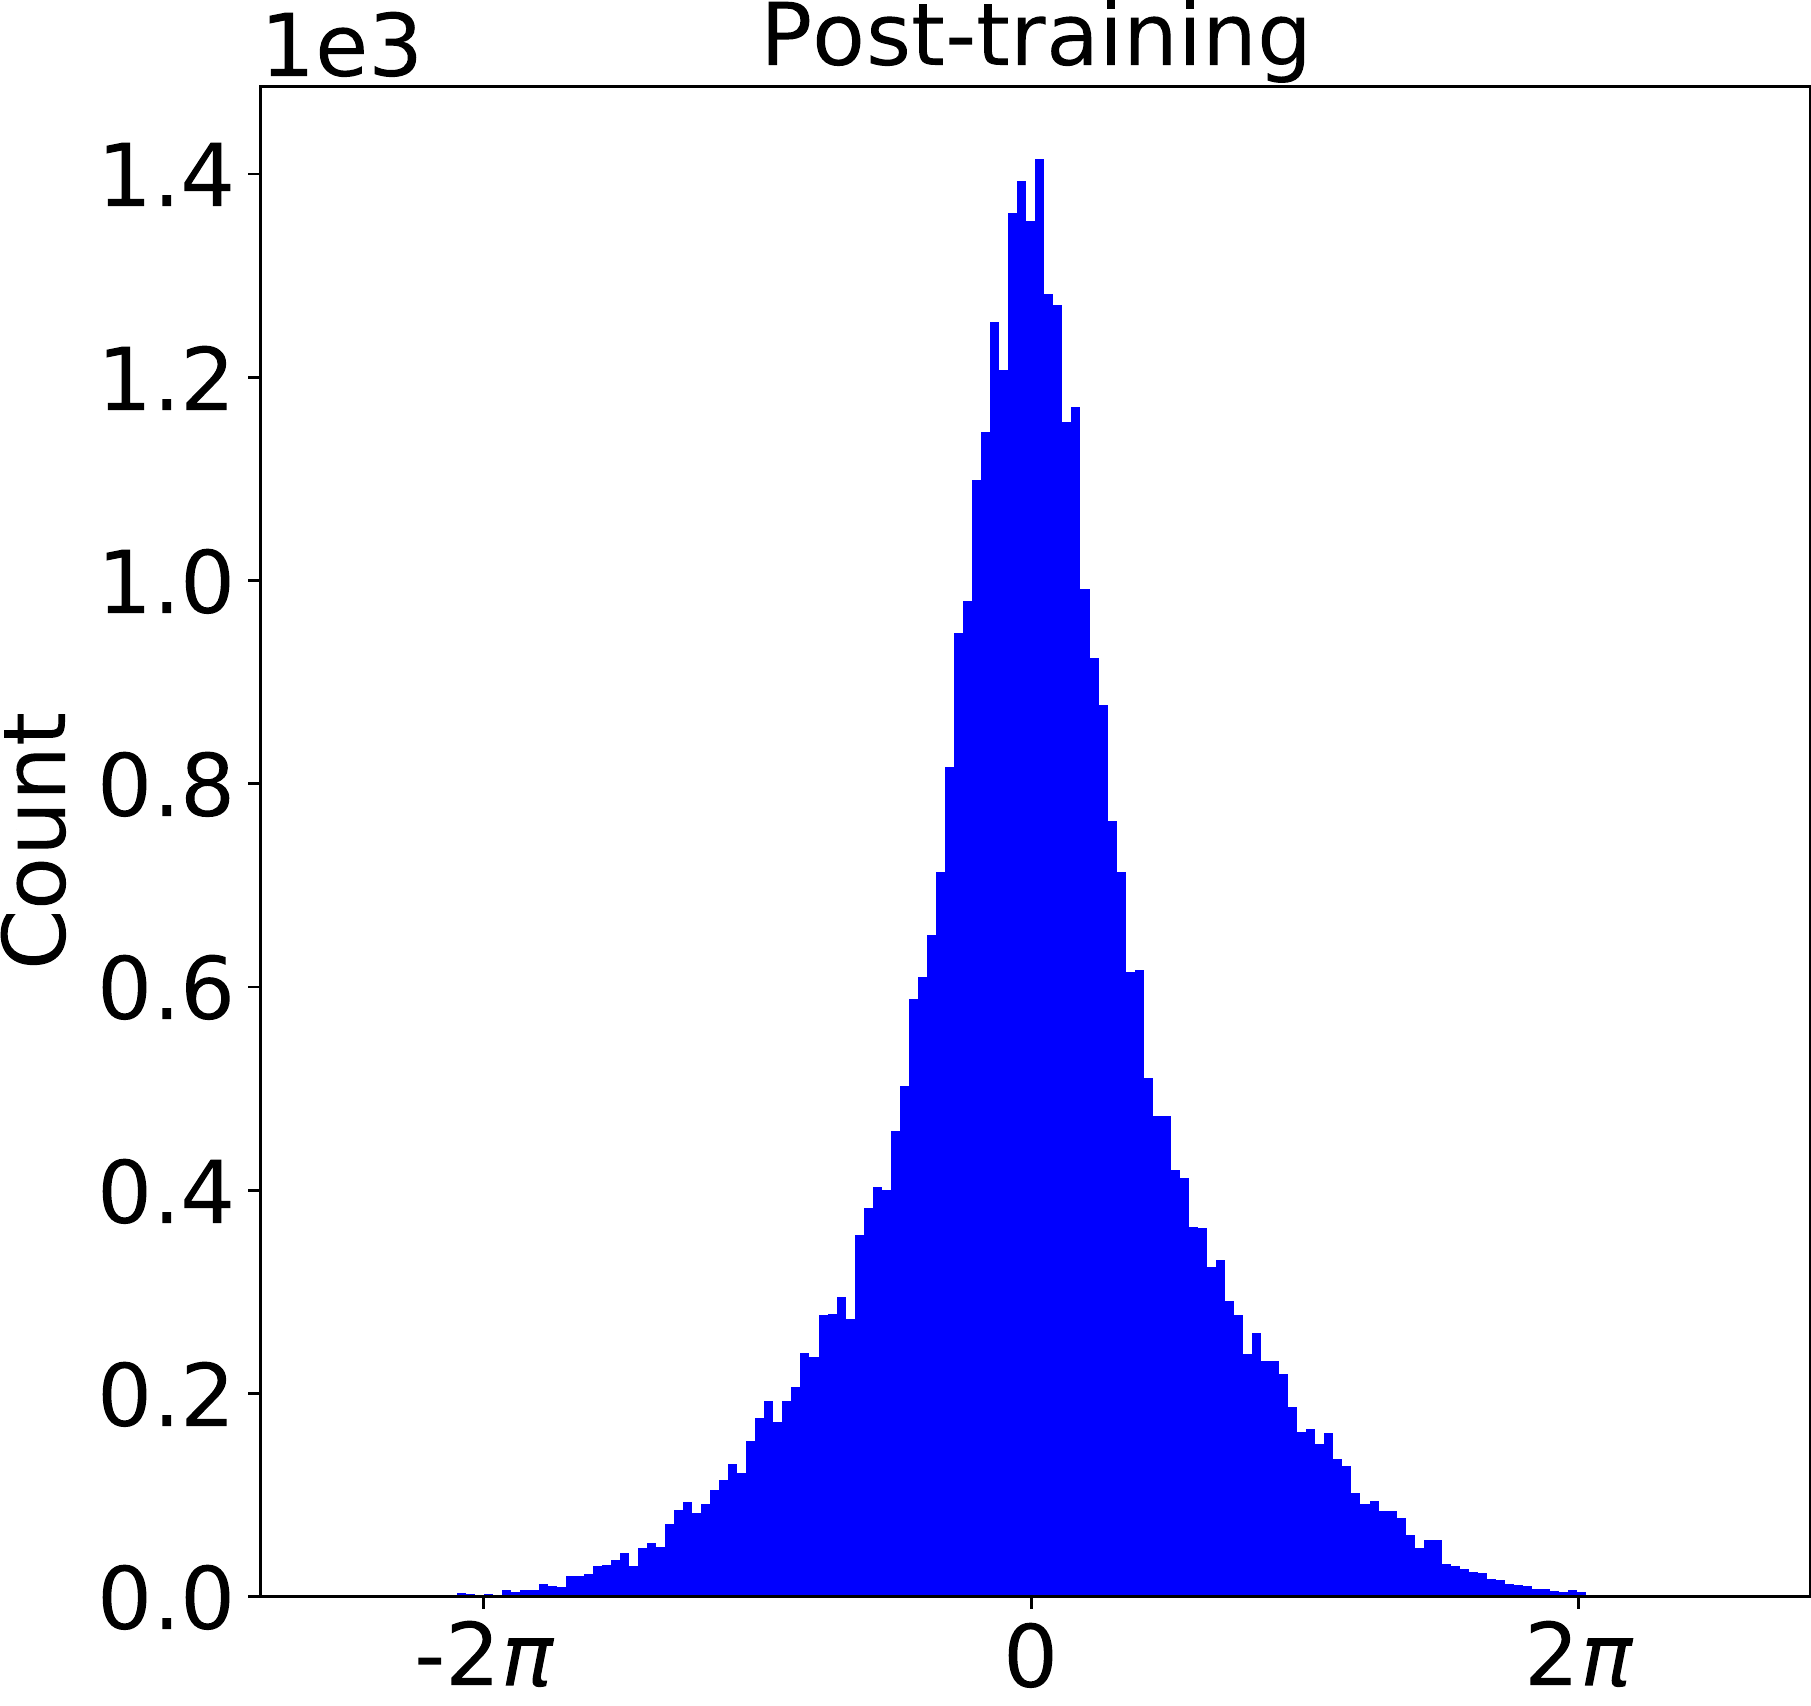}}
        {\includegraphics[width=0.18\linewidth]{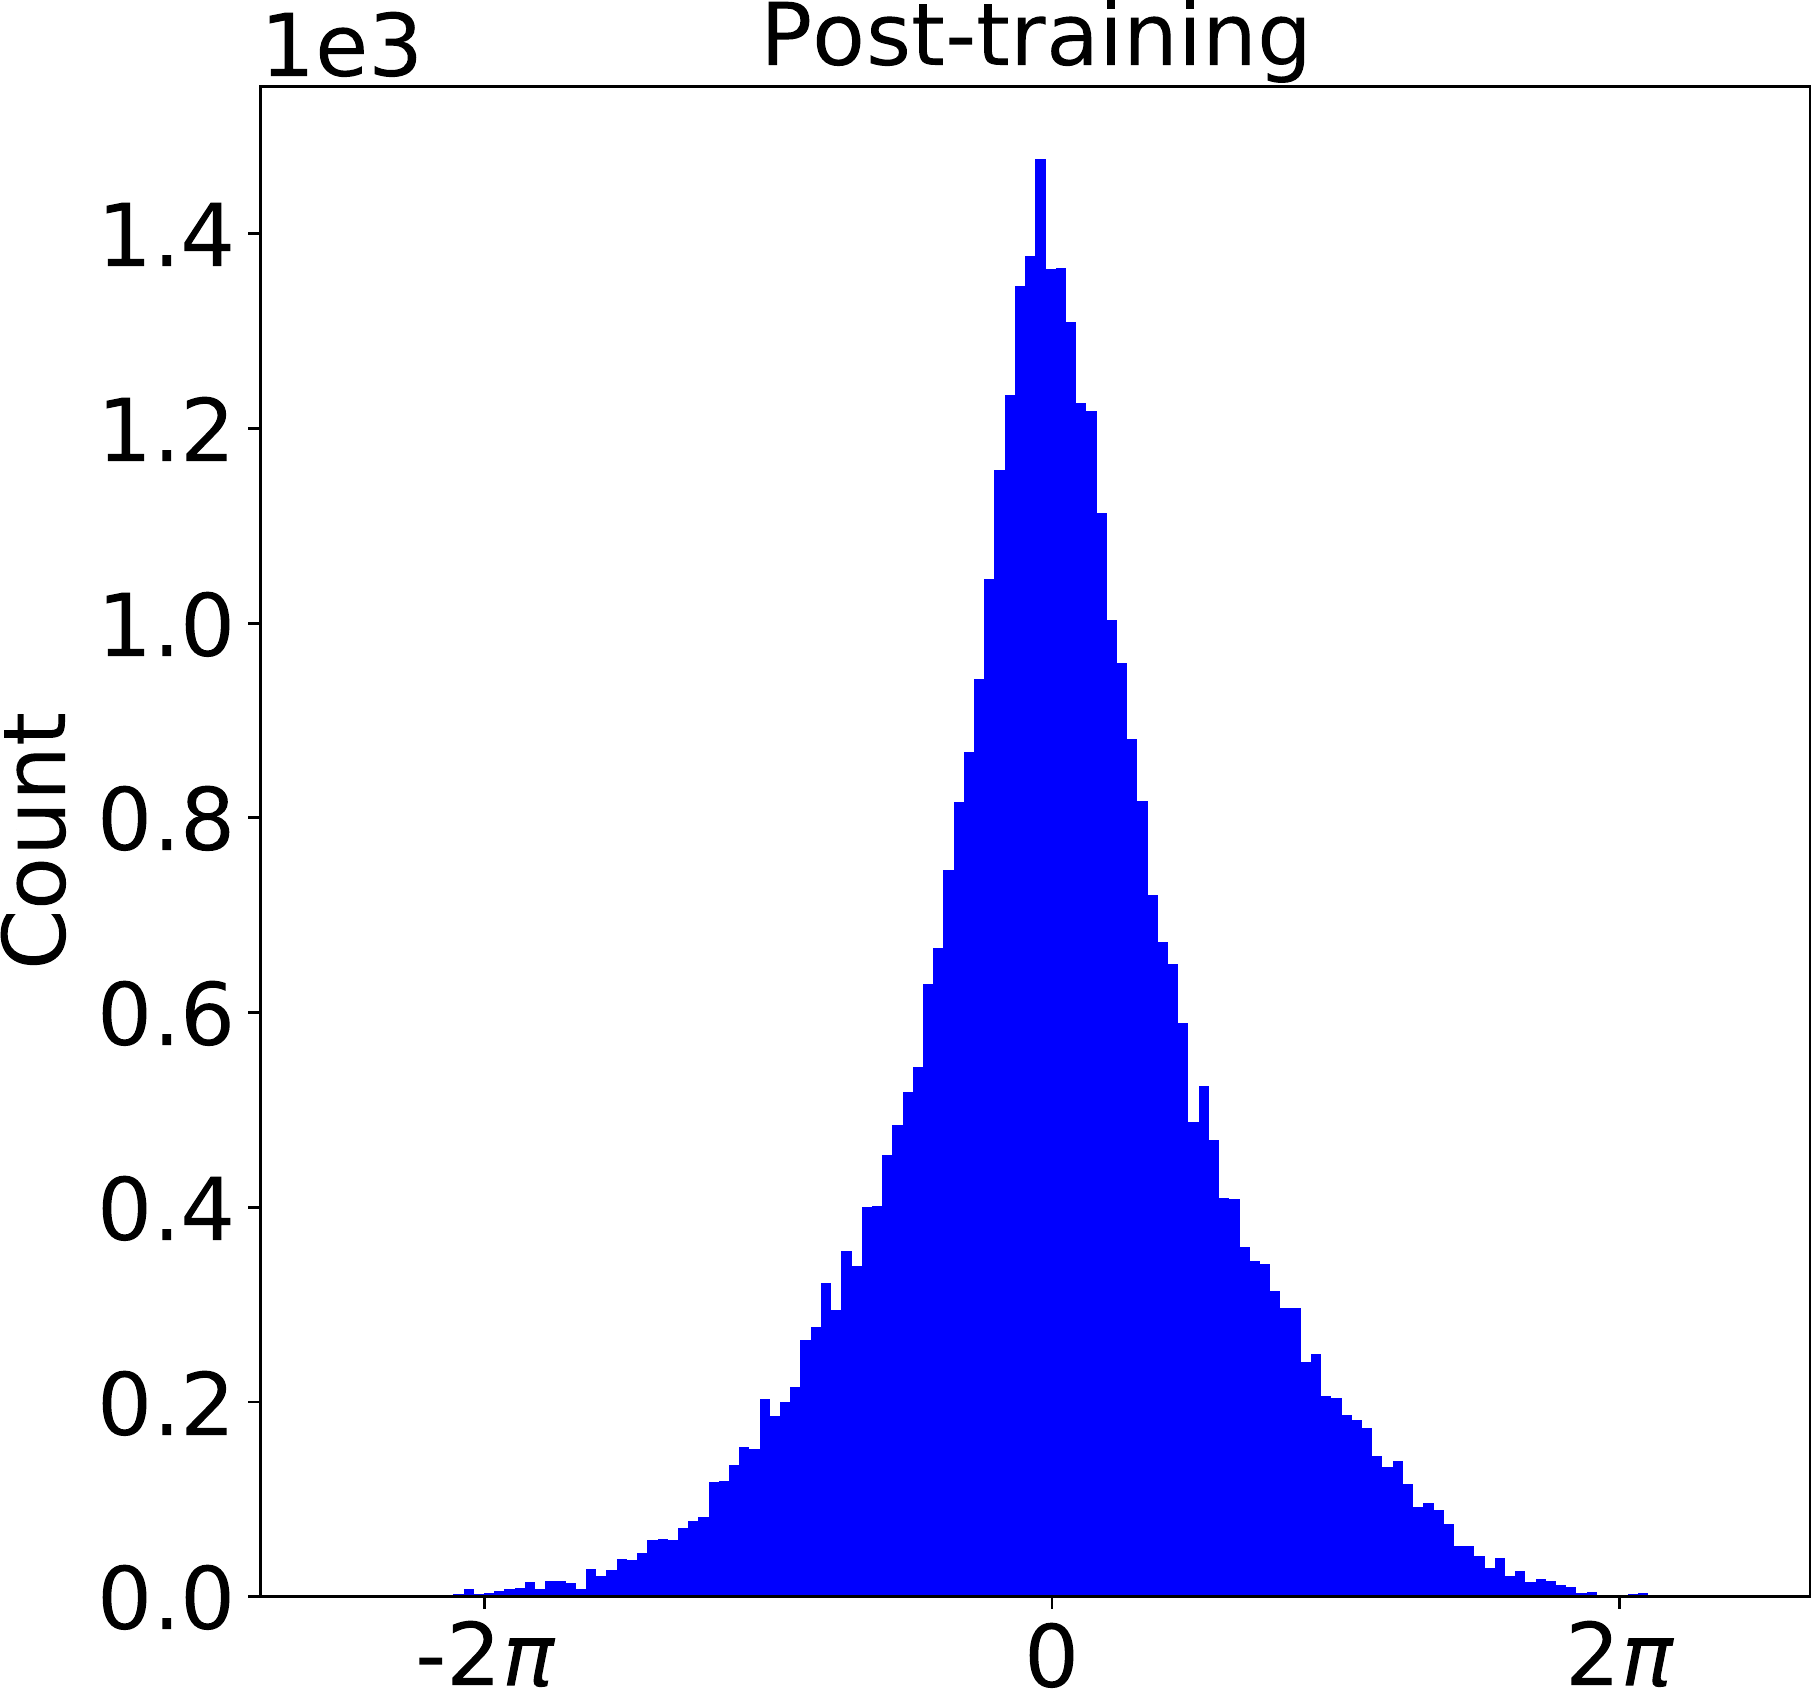}}
        {\includegraphics[width=0.18\linewidth]{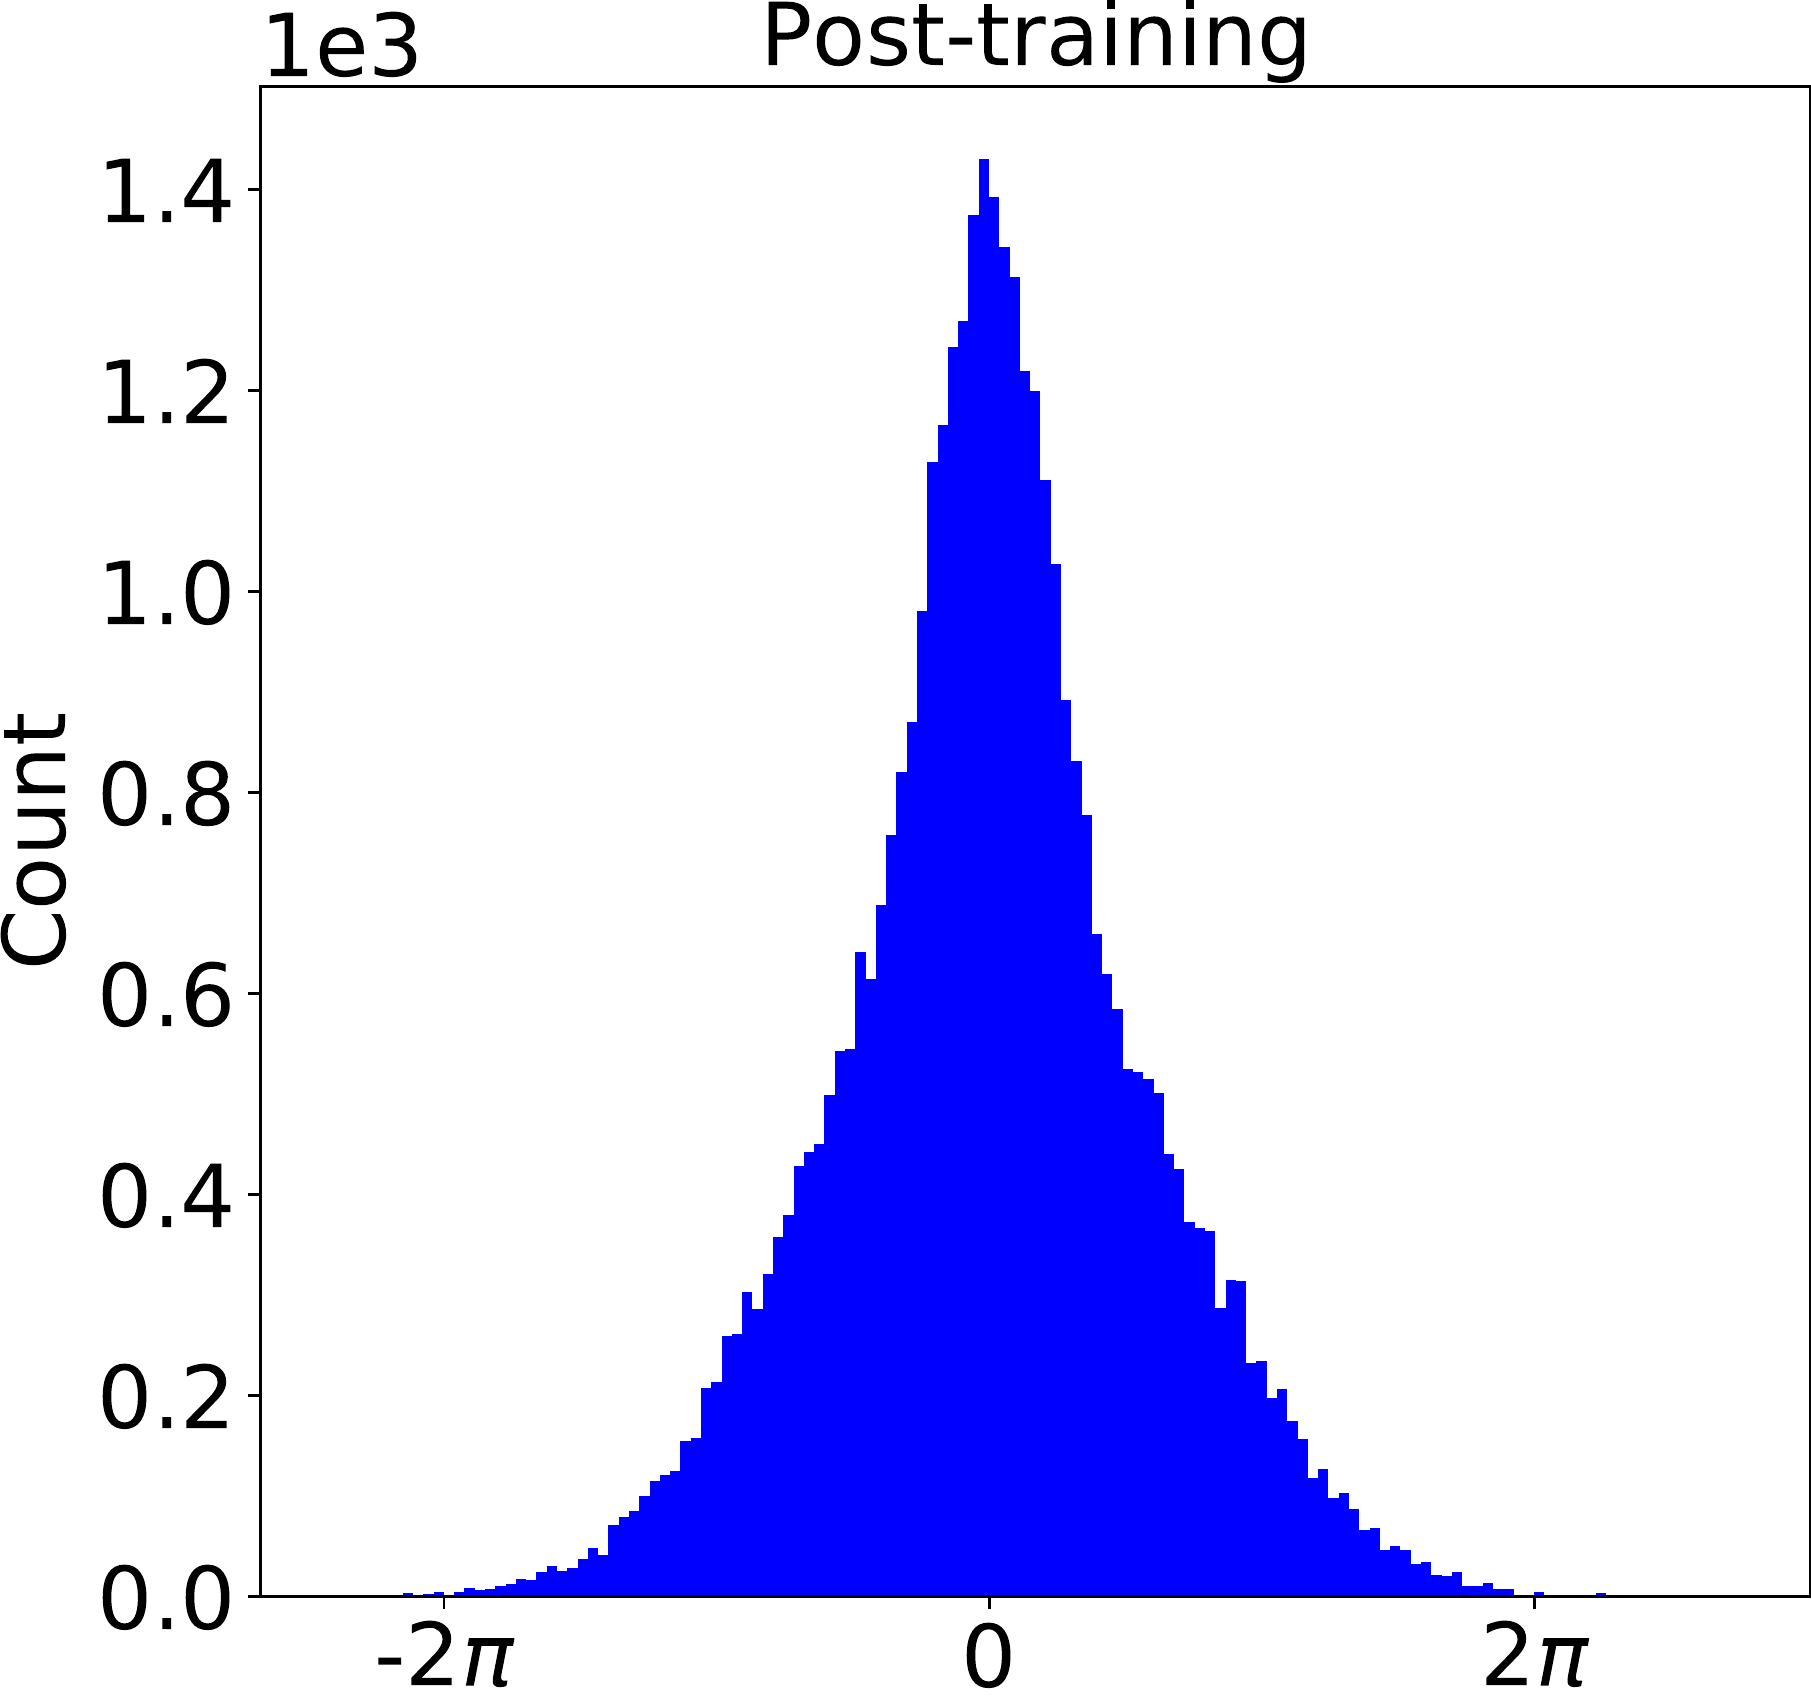}}
        {\includegraphics[width=0.18\linewidth]{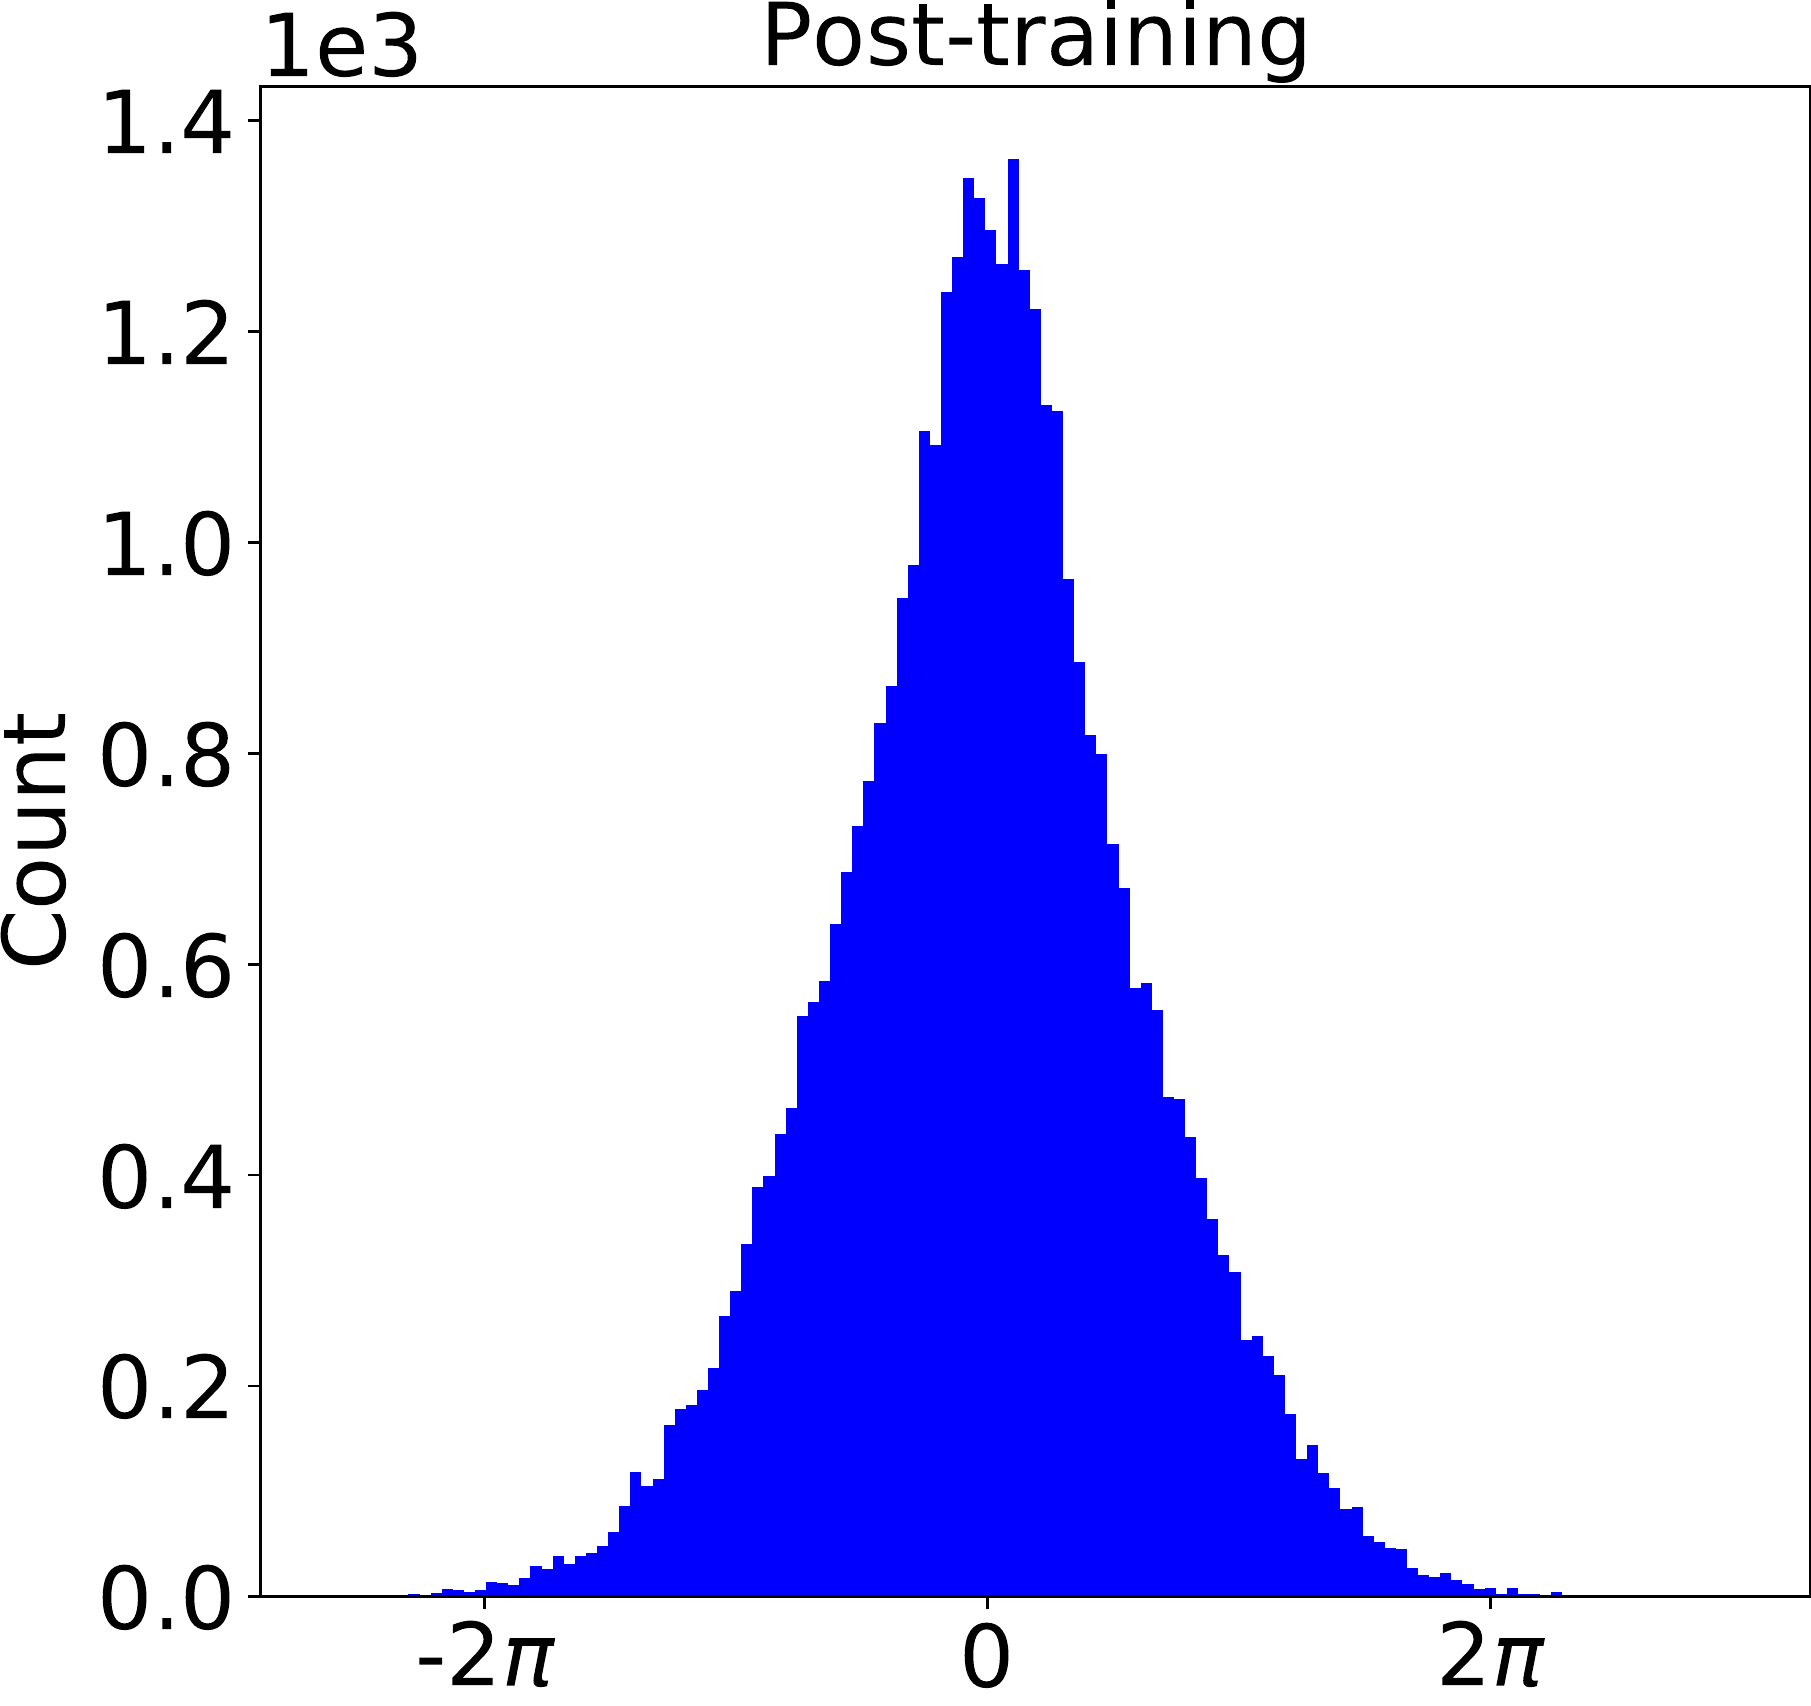}}
        \caption{Weight parameters distribution for layers from first to last in model trained with full precision, shown from left to right.}
    \end{subfigure}
    \hfill
        \begin{subfigure}[b]{1\linewidth}
    \centering
        {\includegraphics[width=0.18\linewidth]{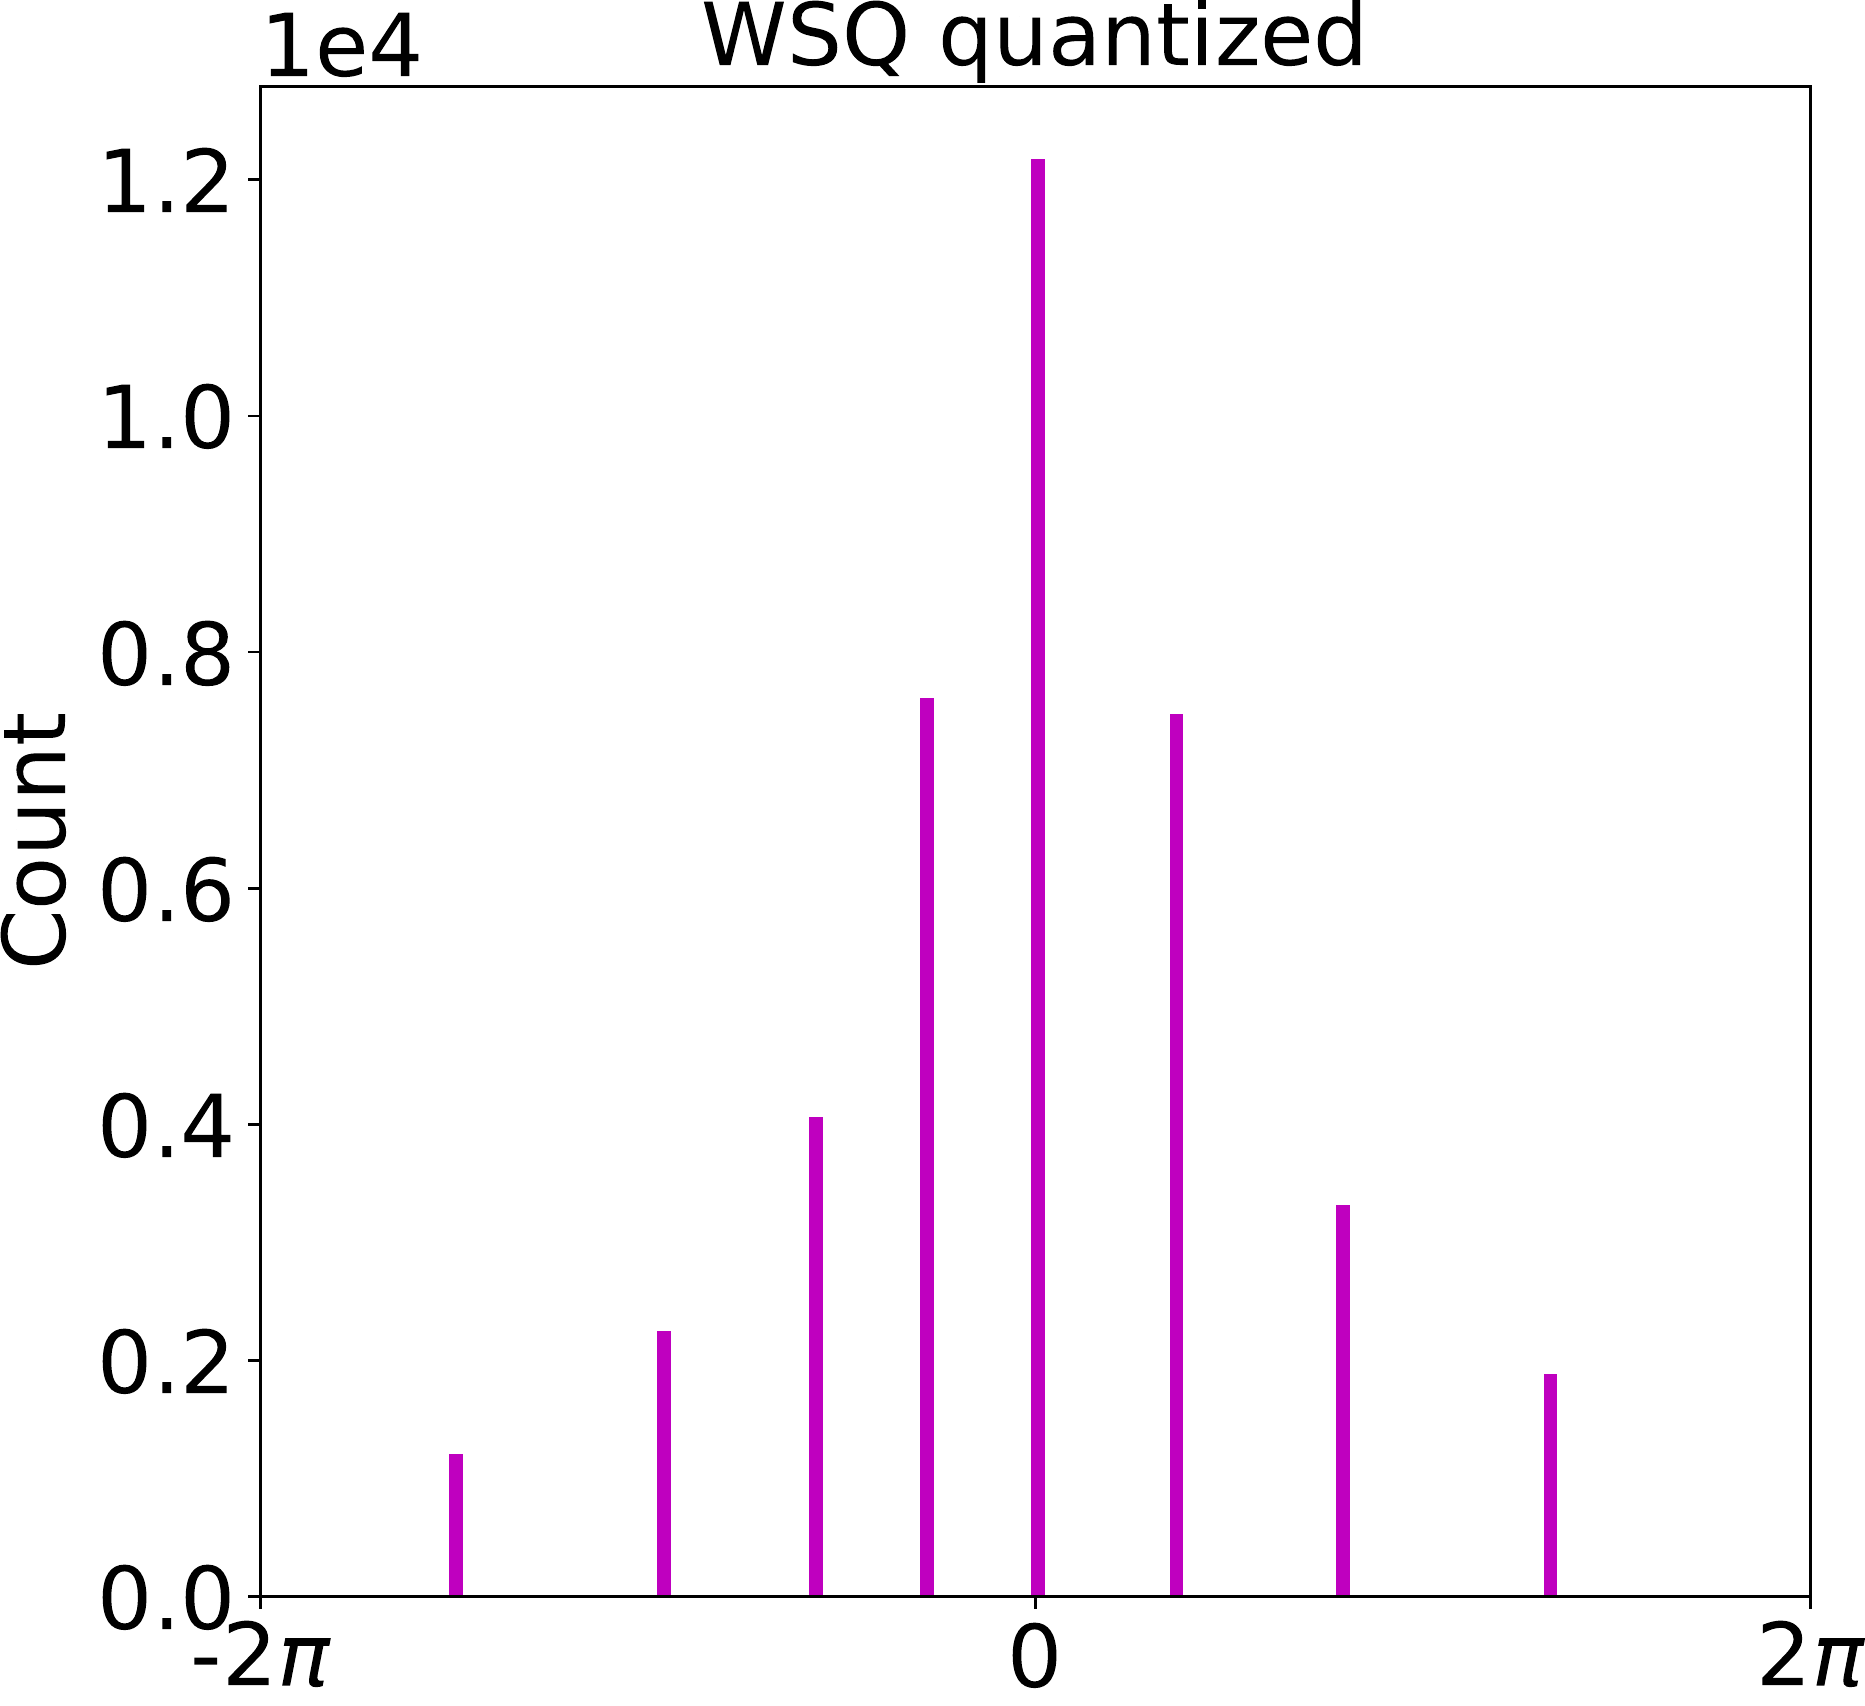}}
        {\includegraphics[width=0.18\linewidth]{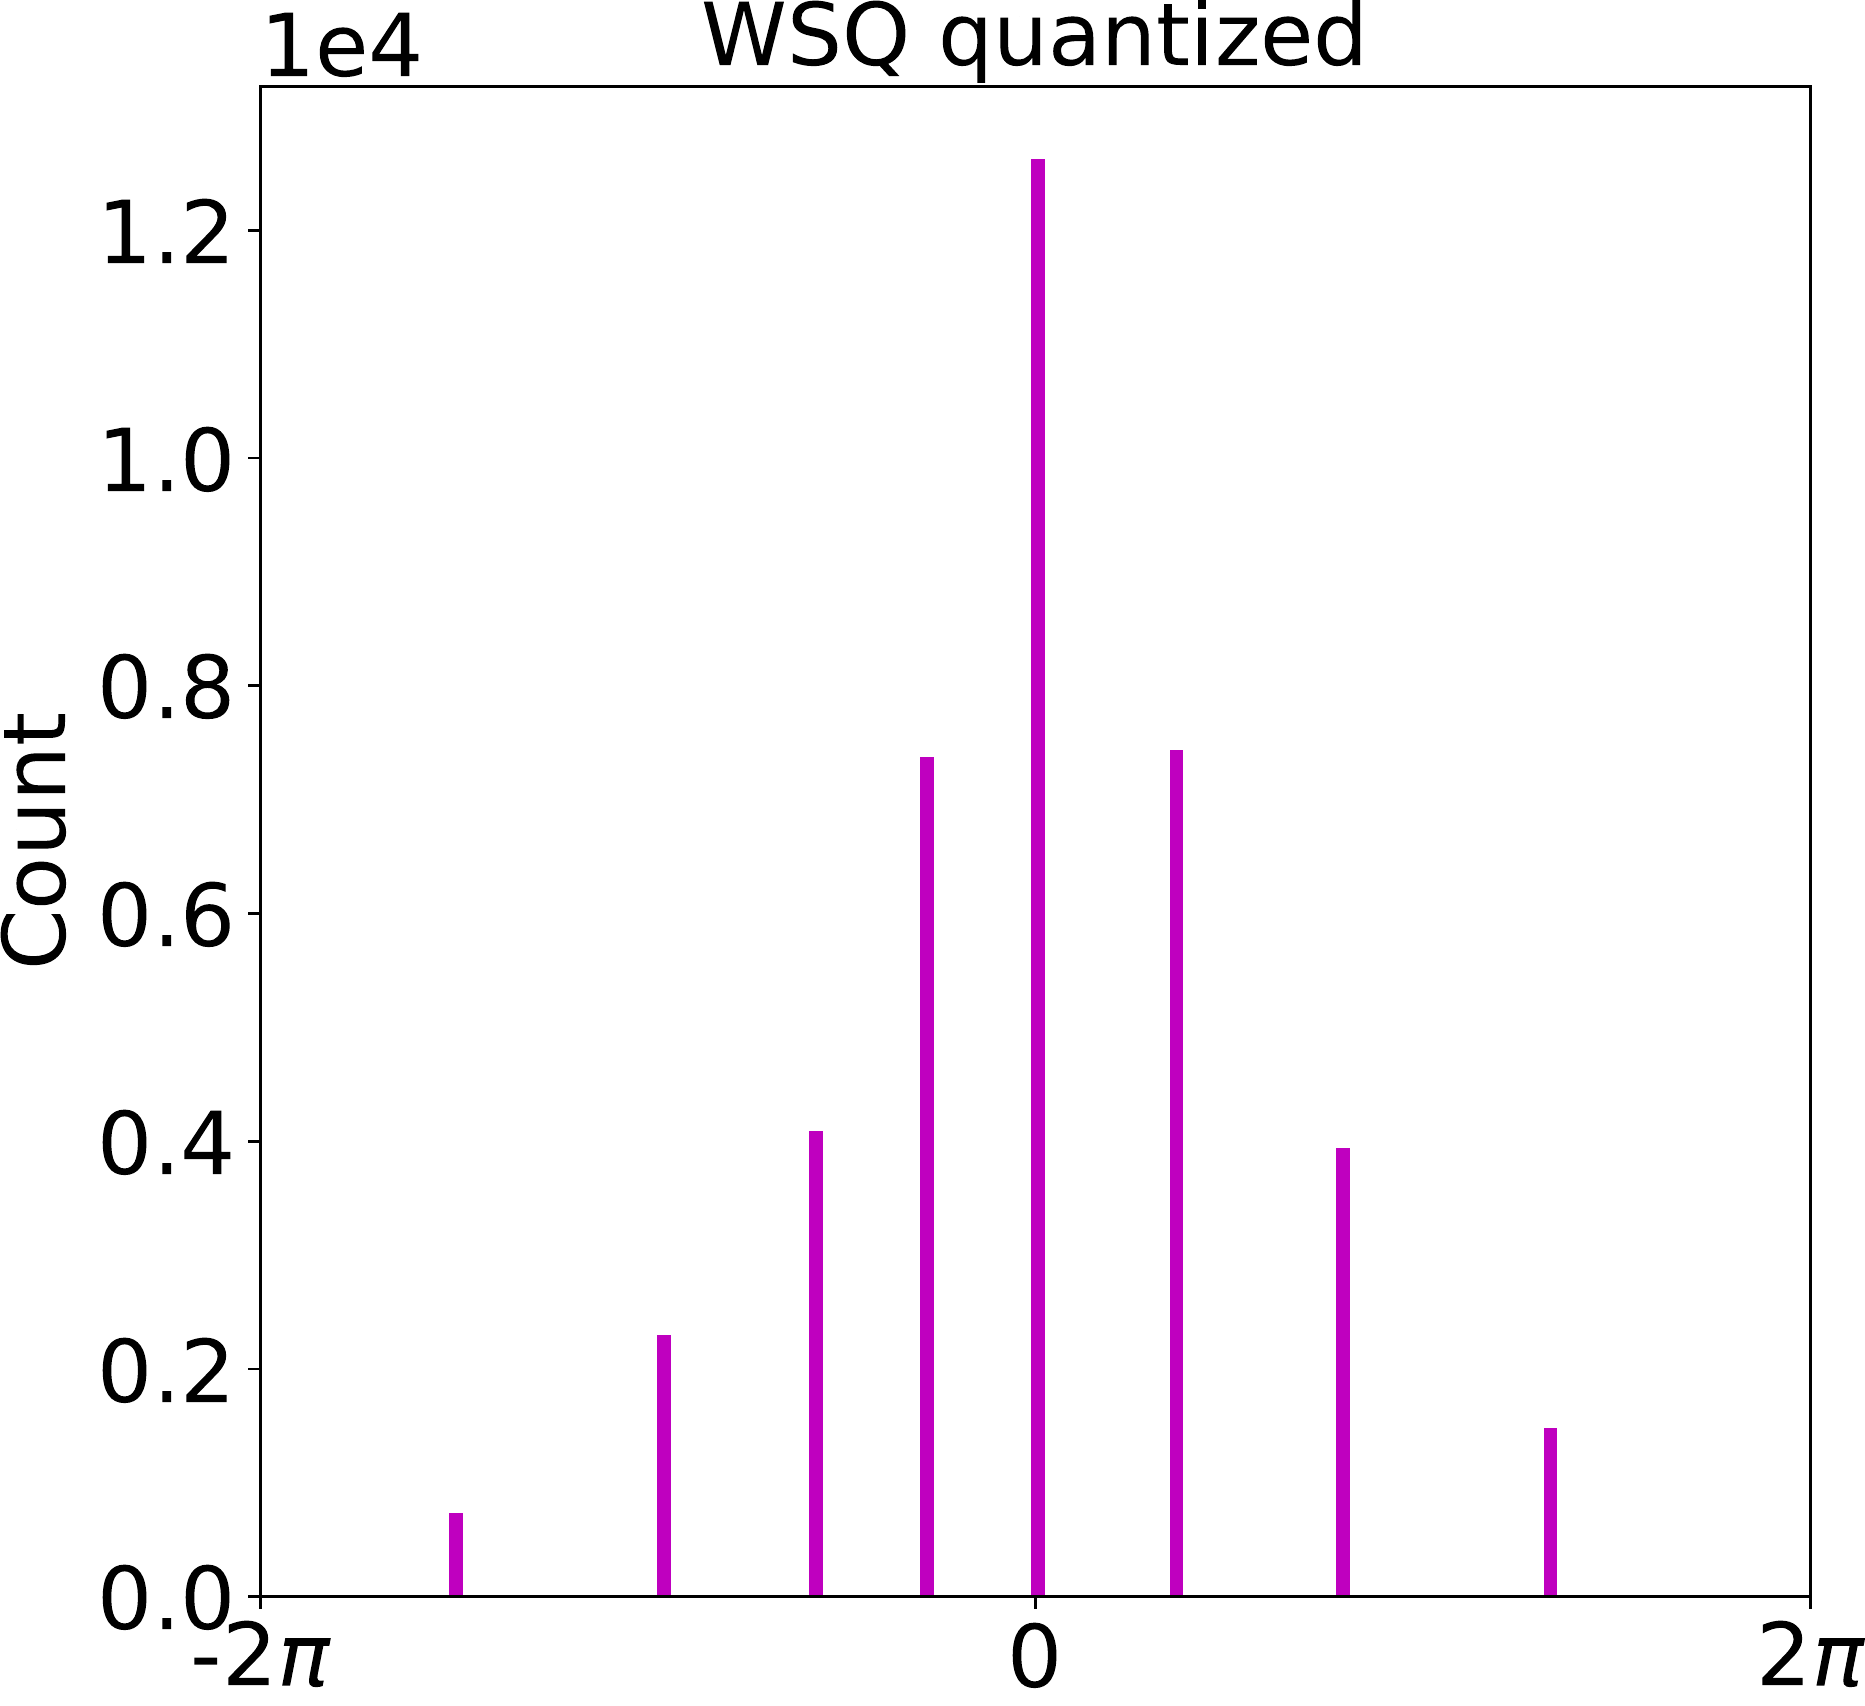}}
        {\includegraphics[width=0.18\linewidth]{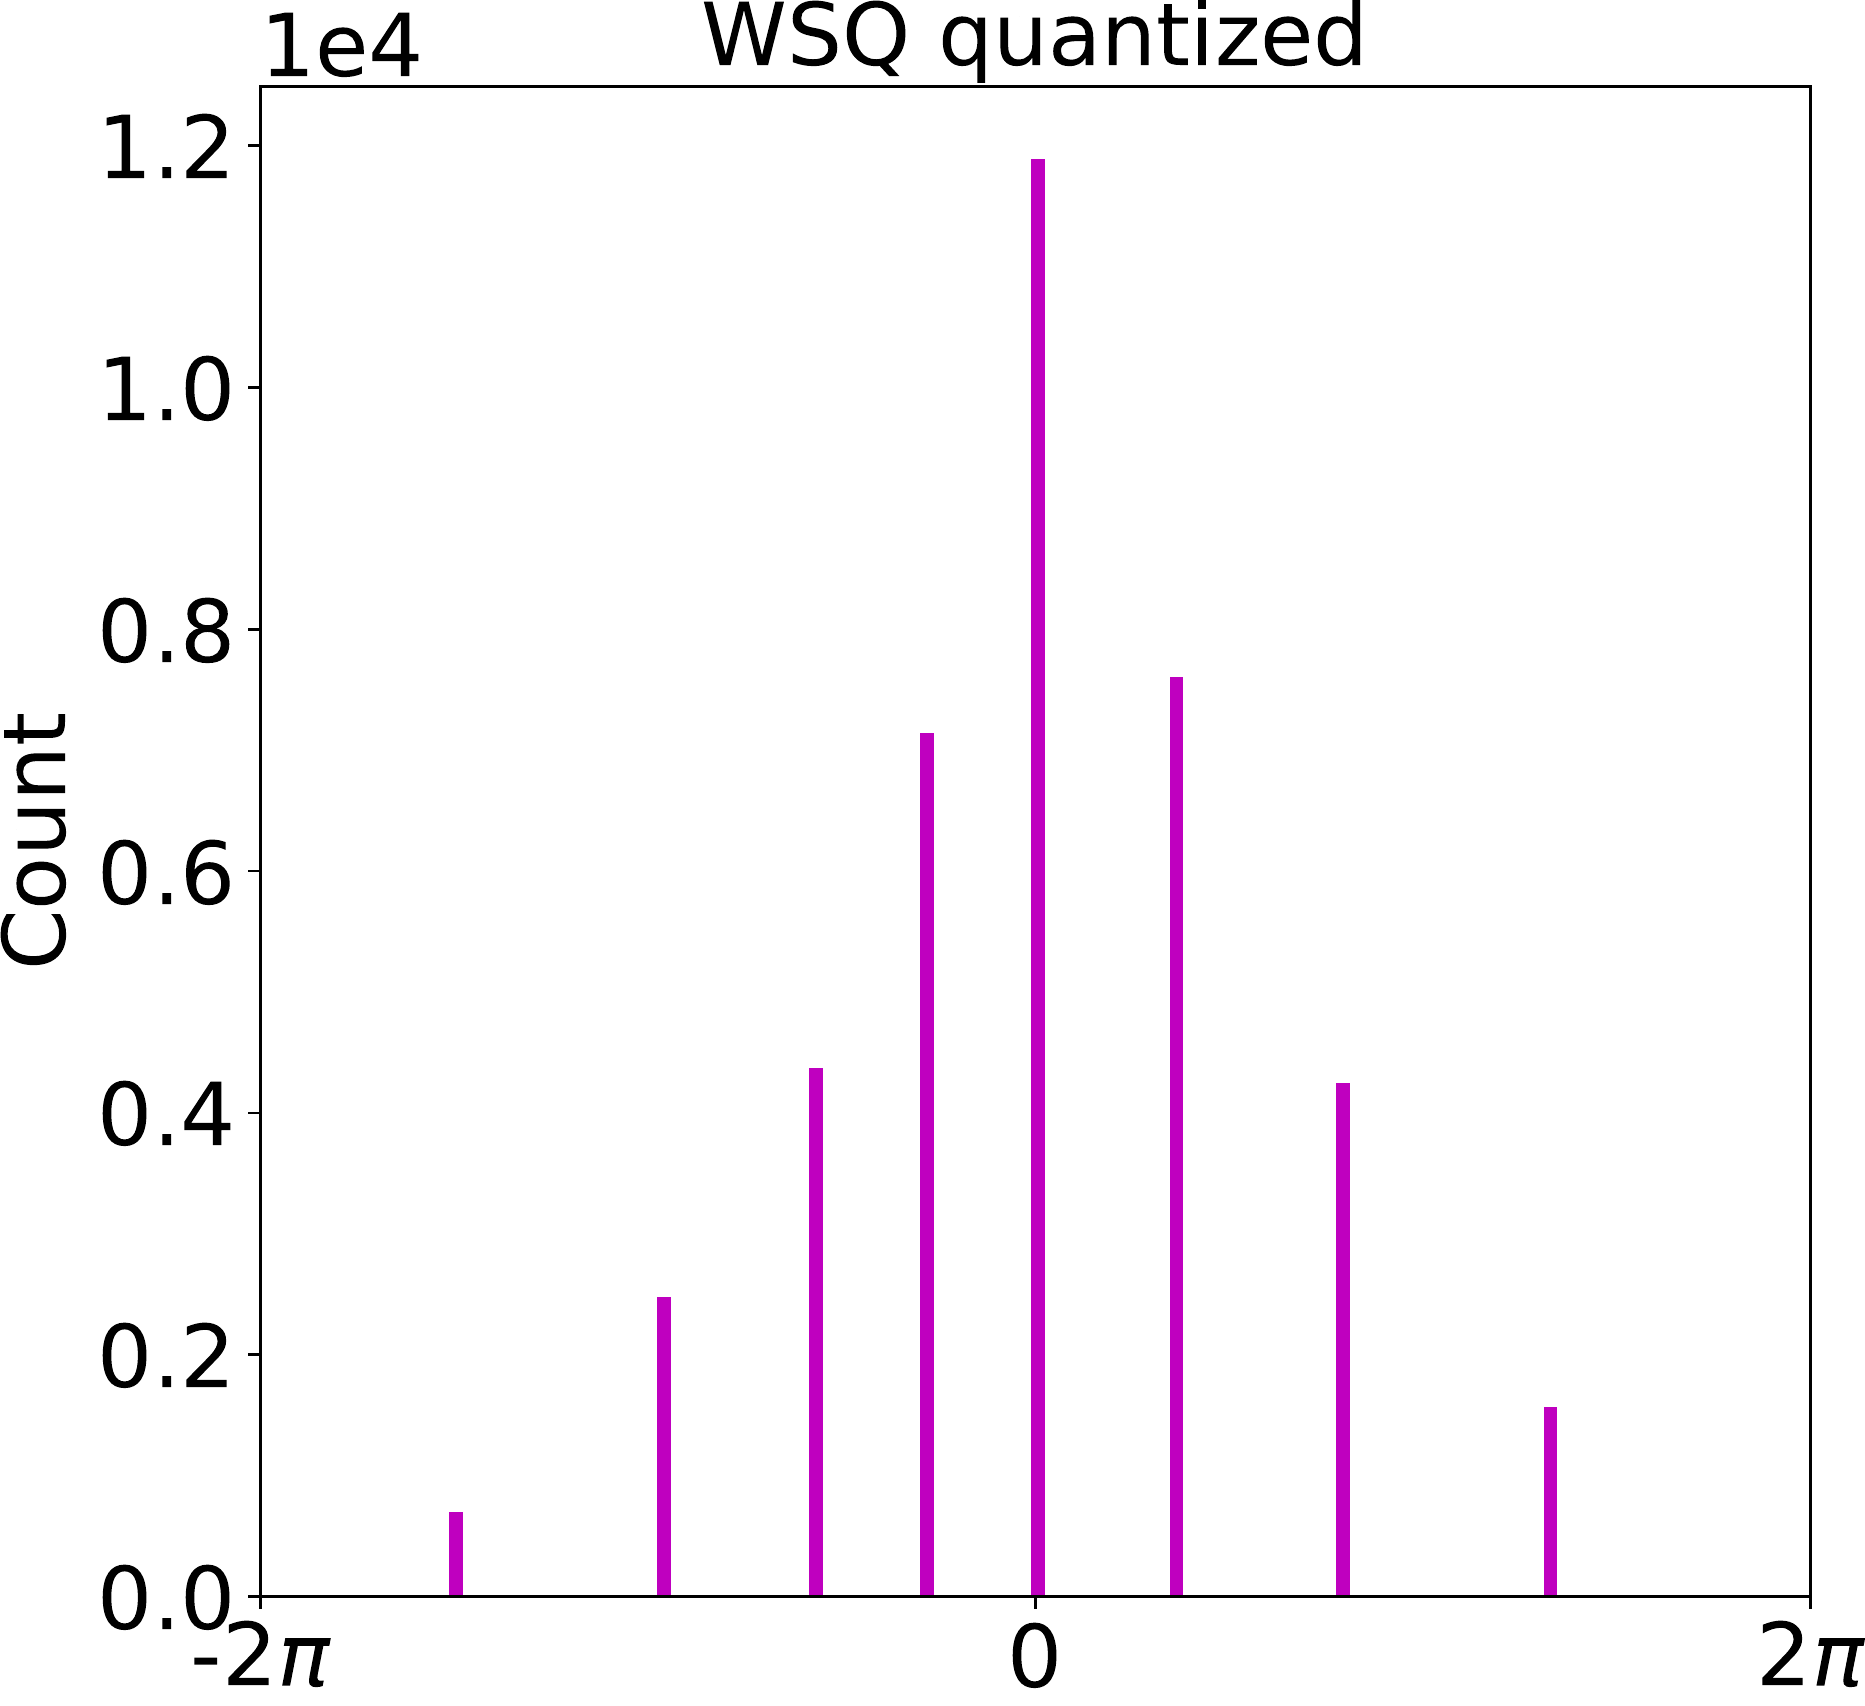}}
        {\includegraphics[width=0.18\linewidth]{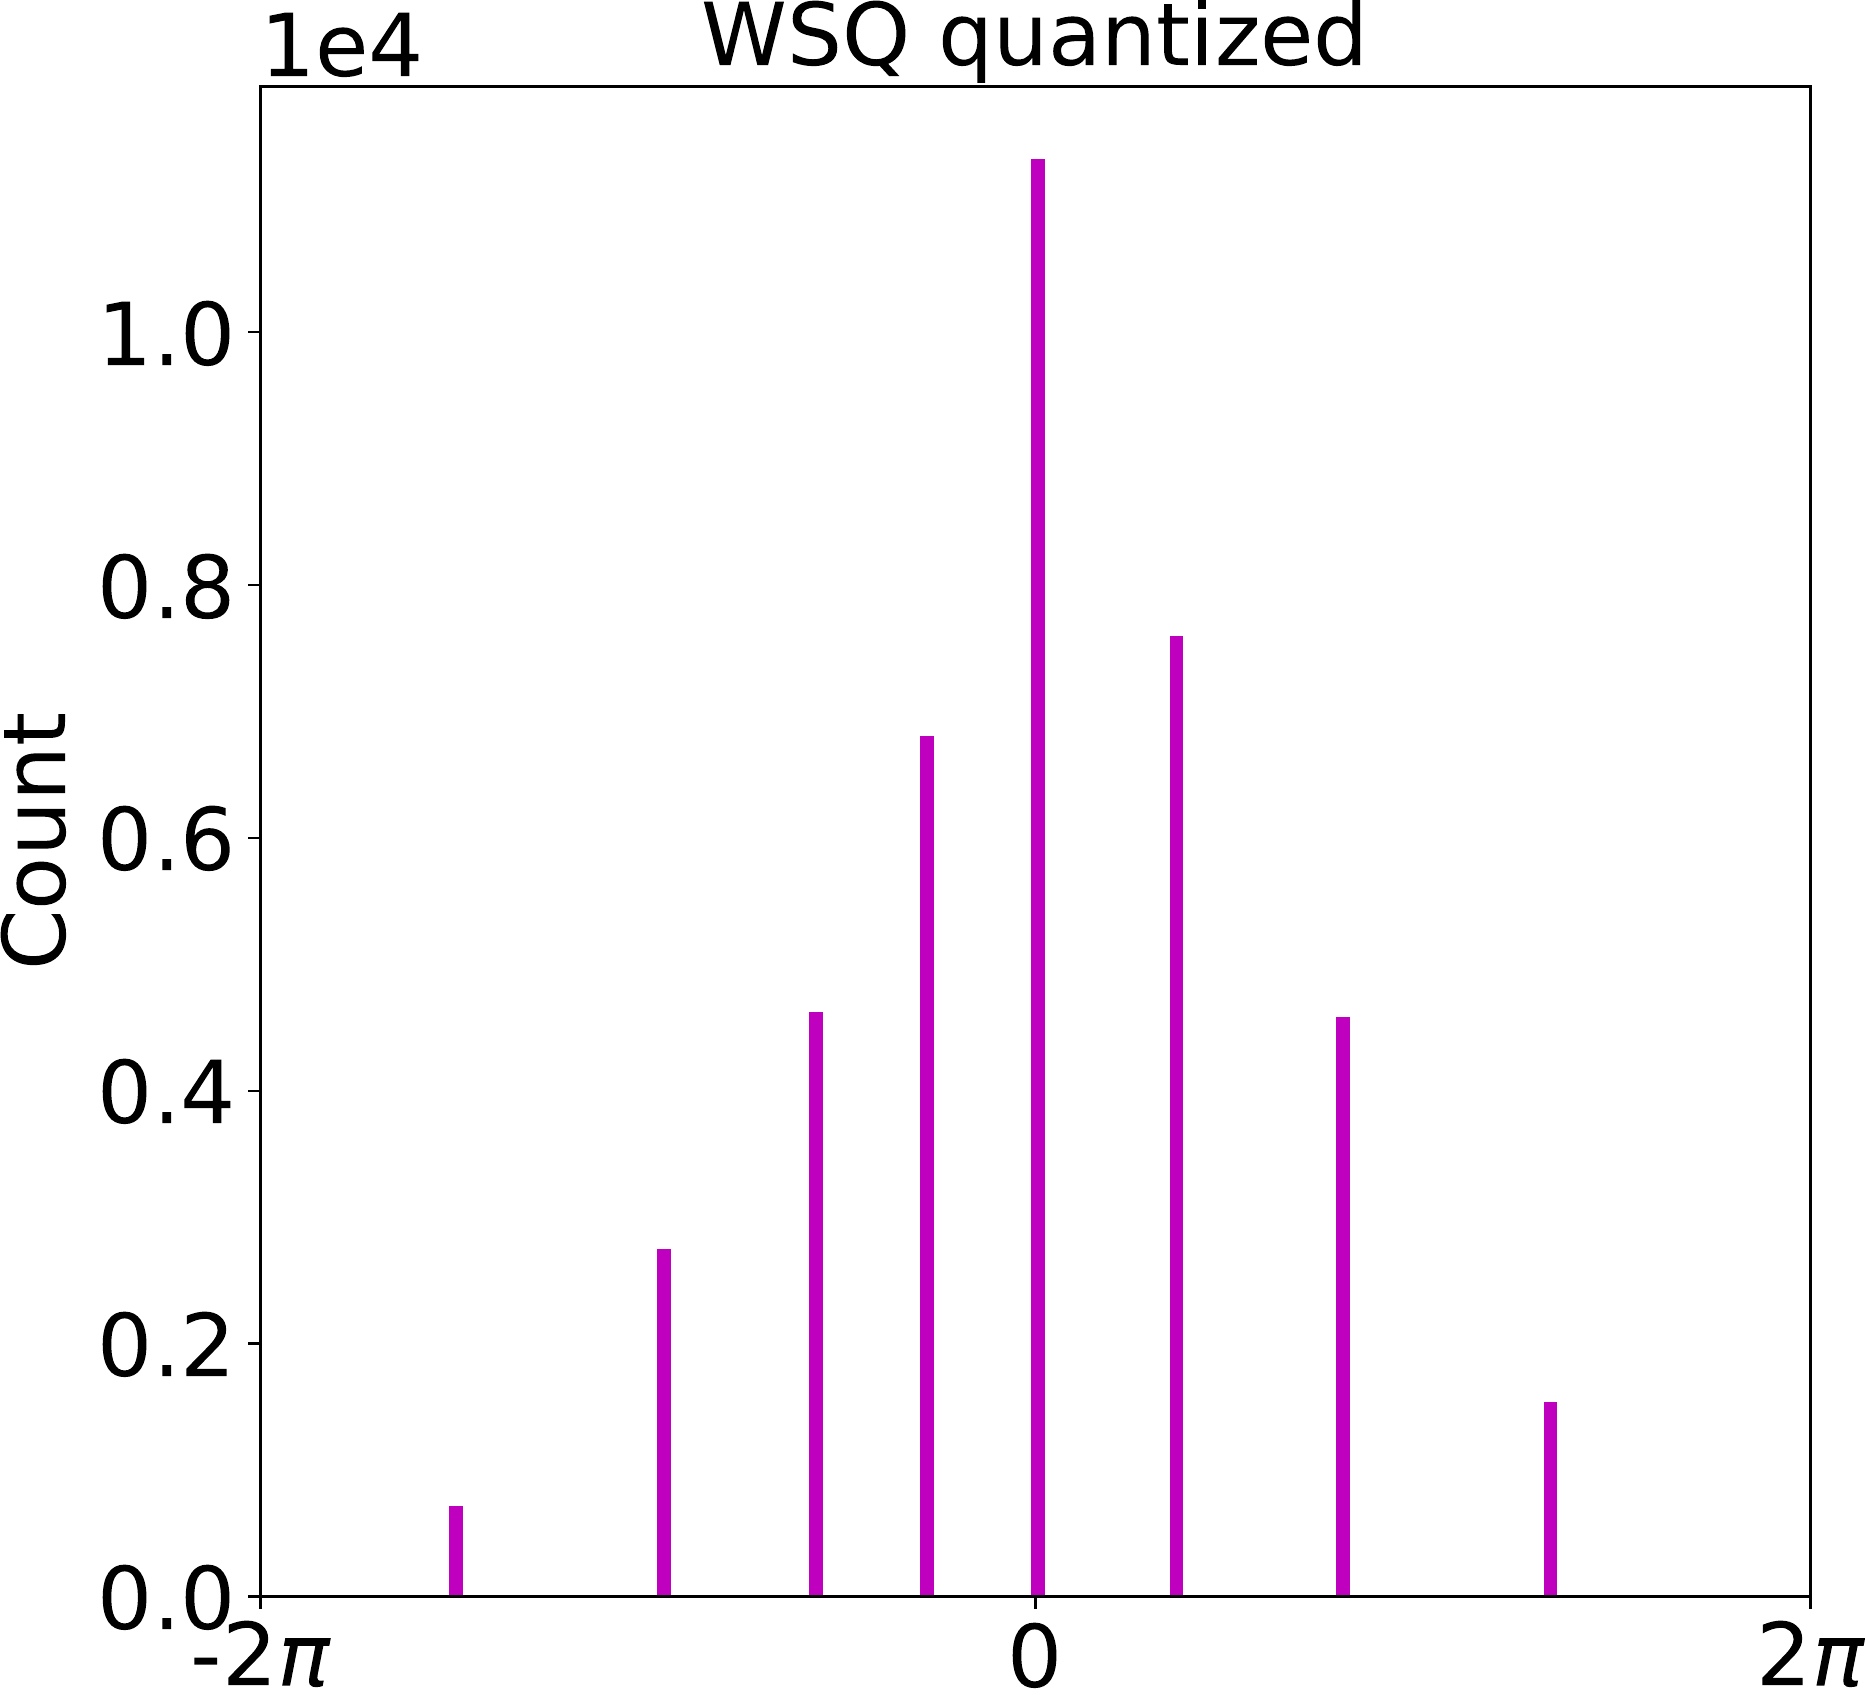}}
        {\includegraphics[width=0.18\linewidth]{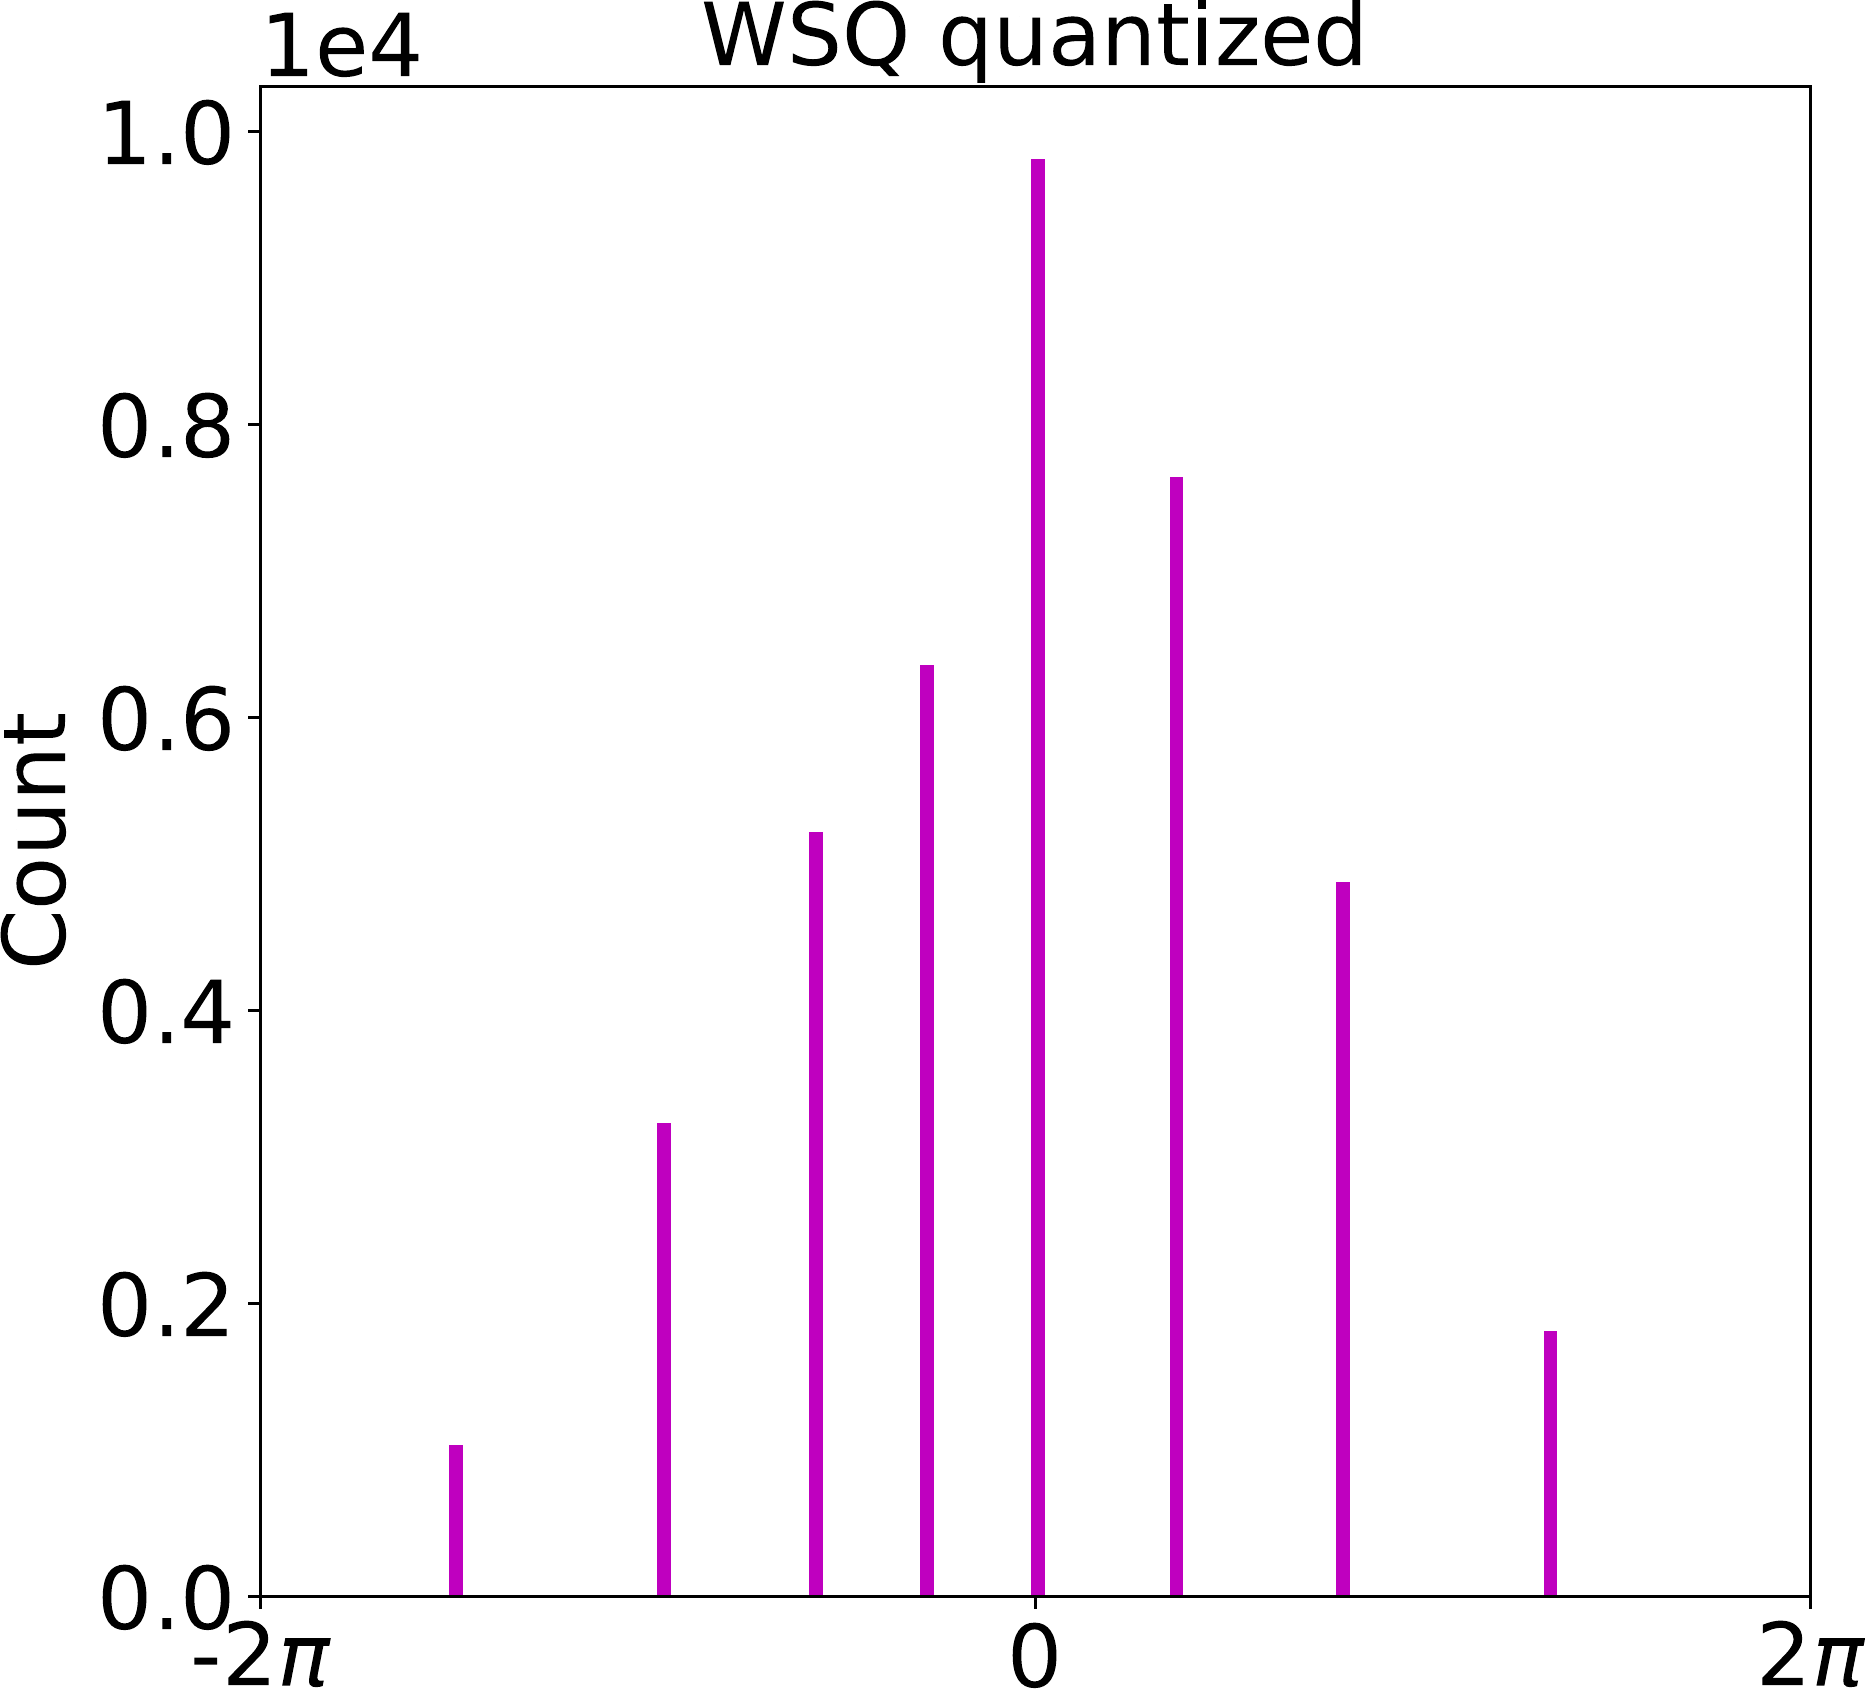}}
        \caption{Weight parameters distribution for layers from first to last in model trained with WSQ before post processing, shown from left to right.}
    \end{subfigure}
    \hfill
    \begin{subfigure}[b]{1\linewidth}
    \centering
        {\includegraphics[width=0.18\linewidth]{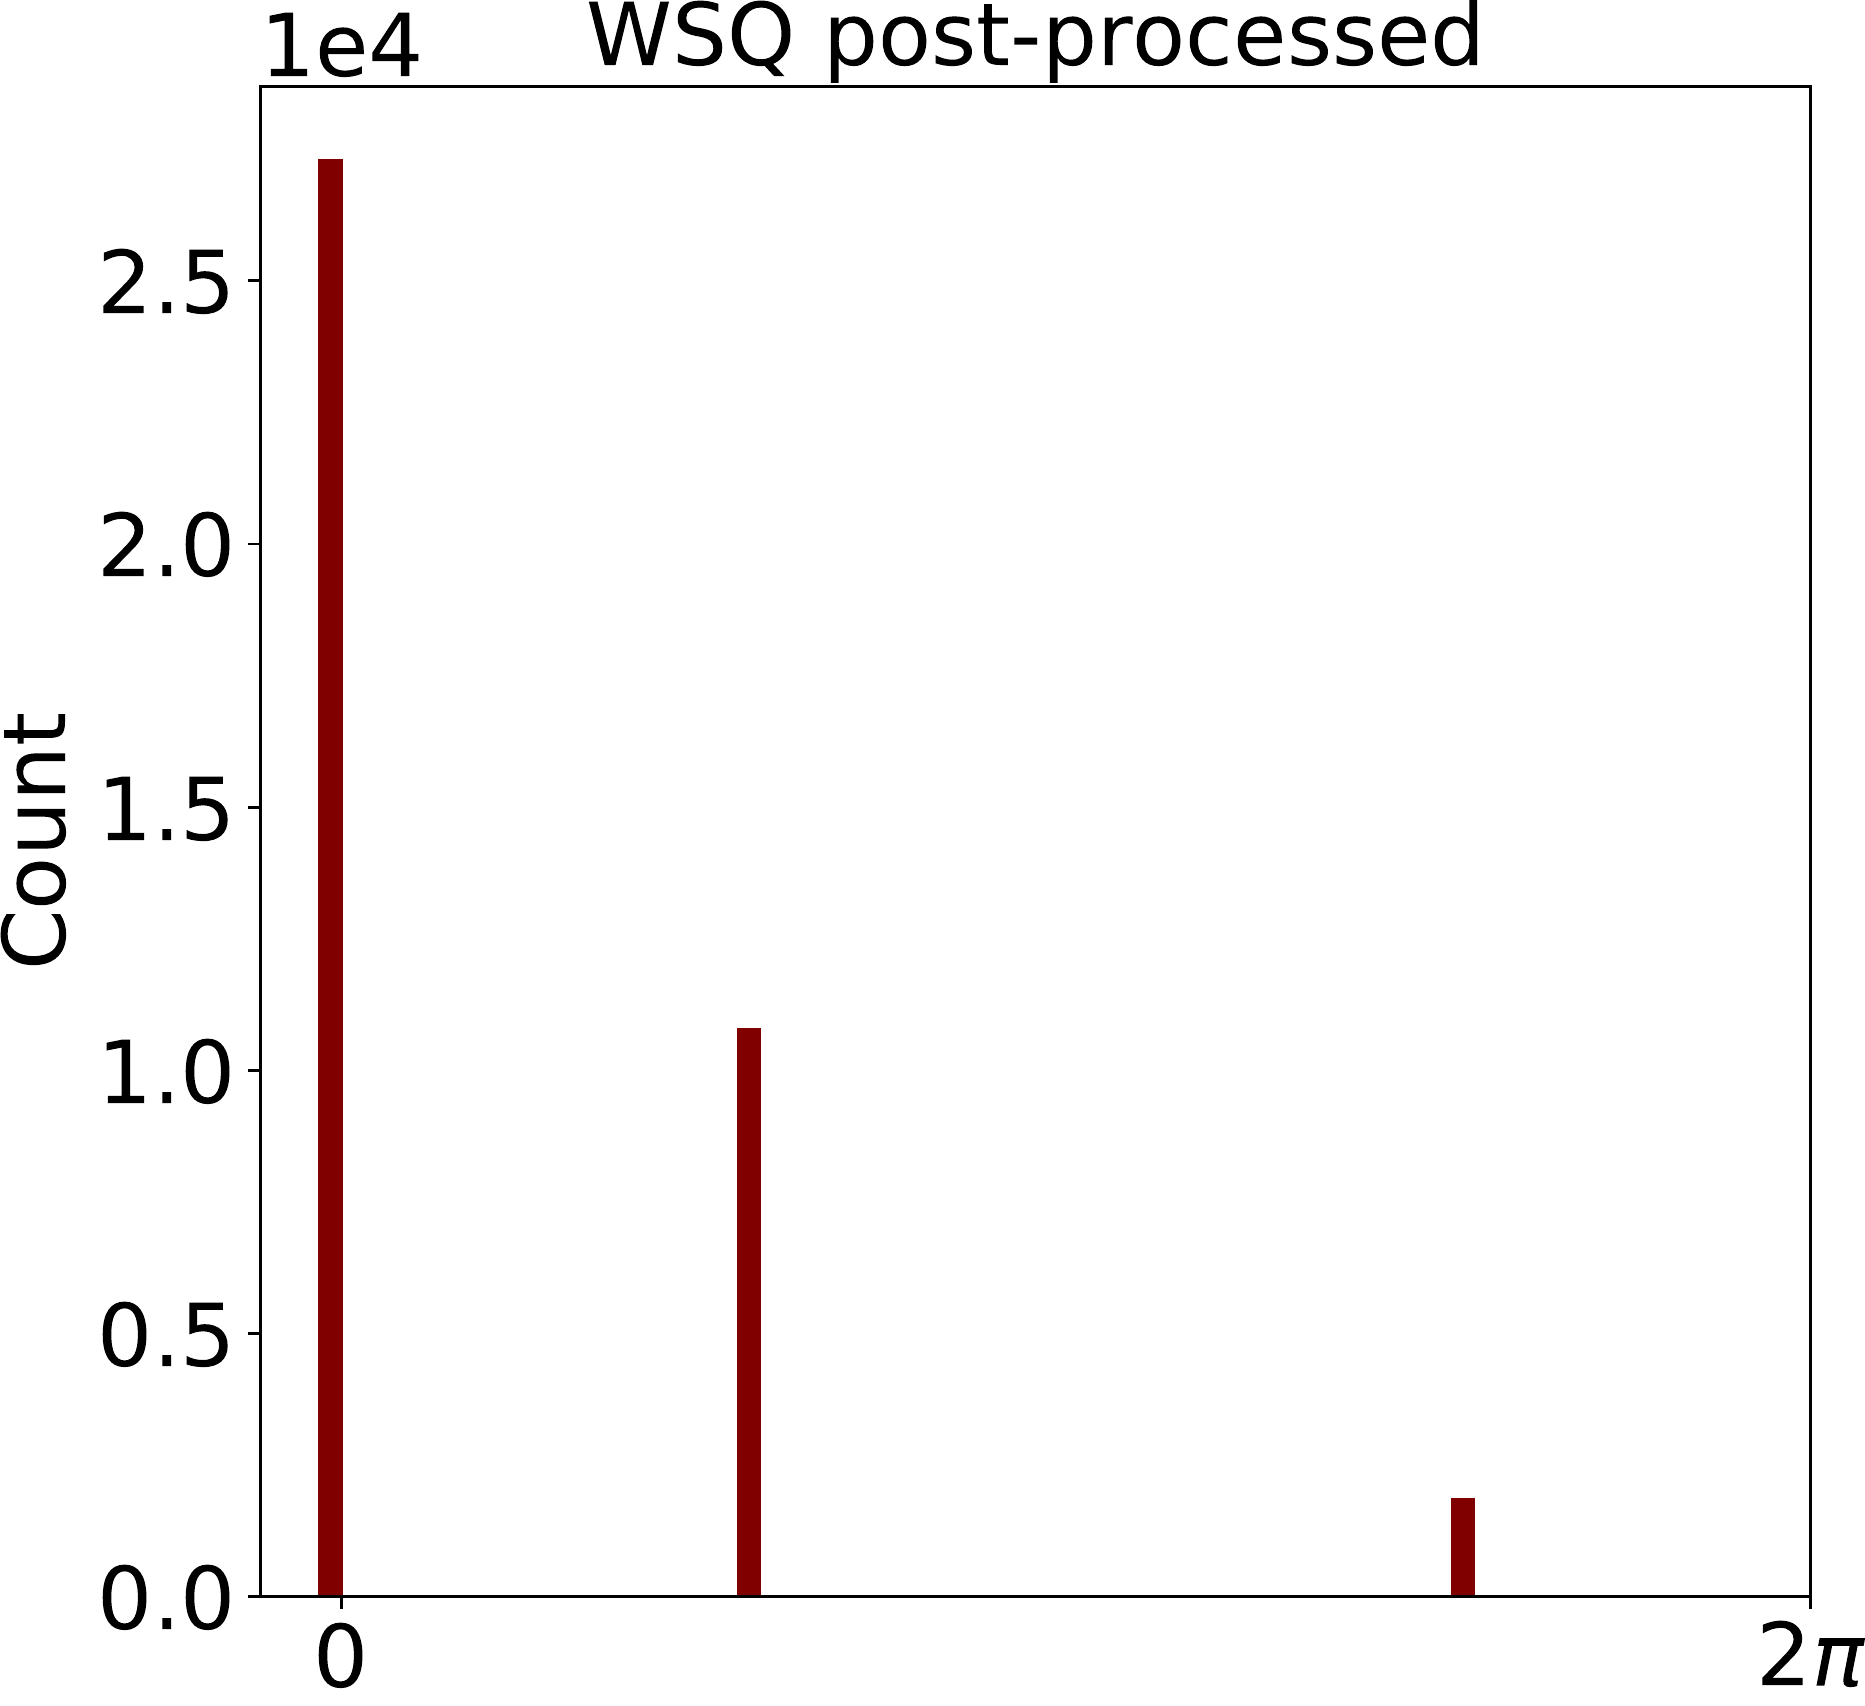}}
        {\includegraphics[width=0.18\linewidth]{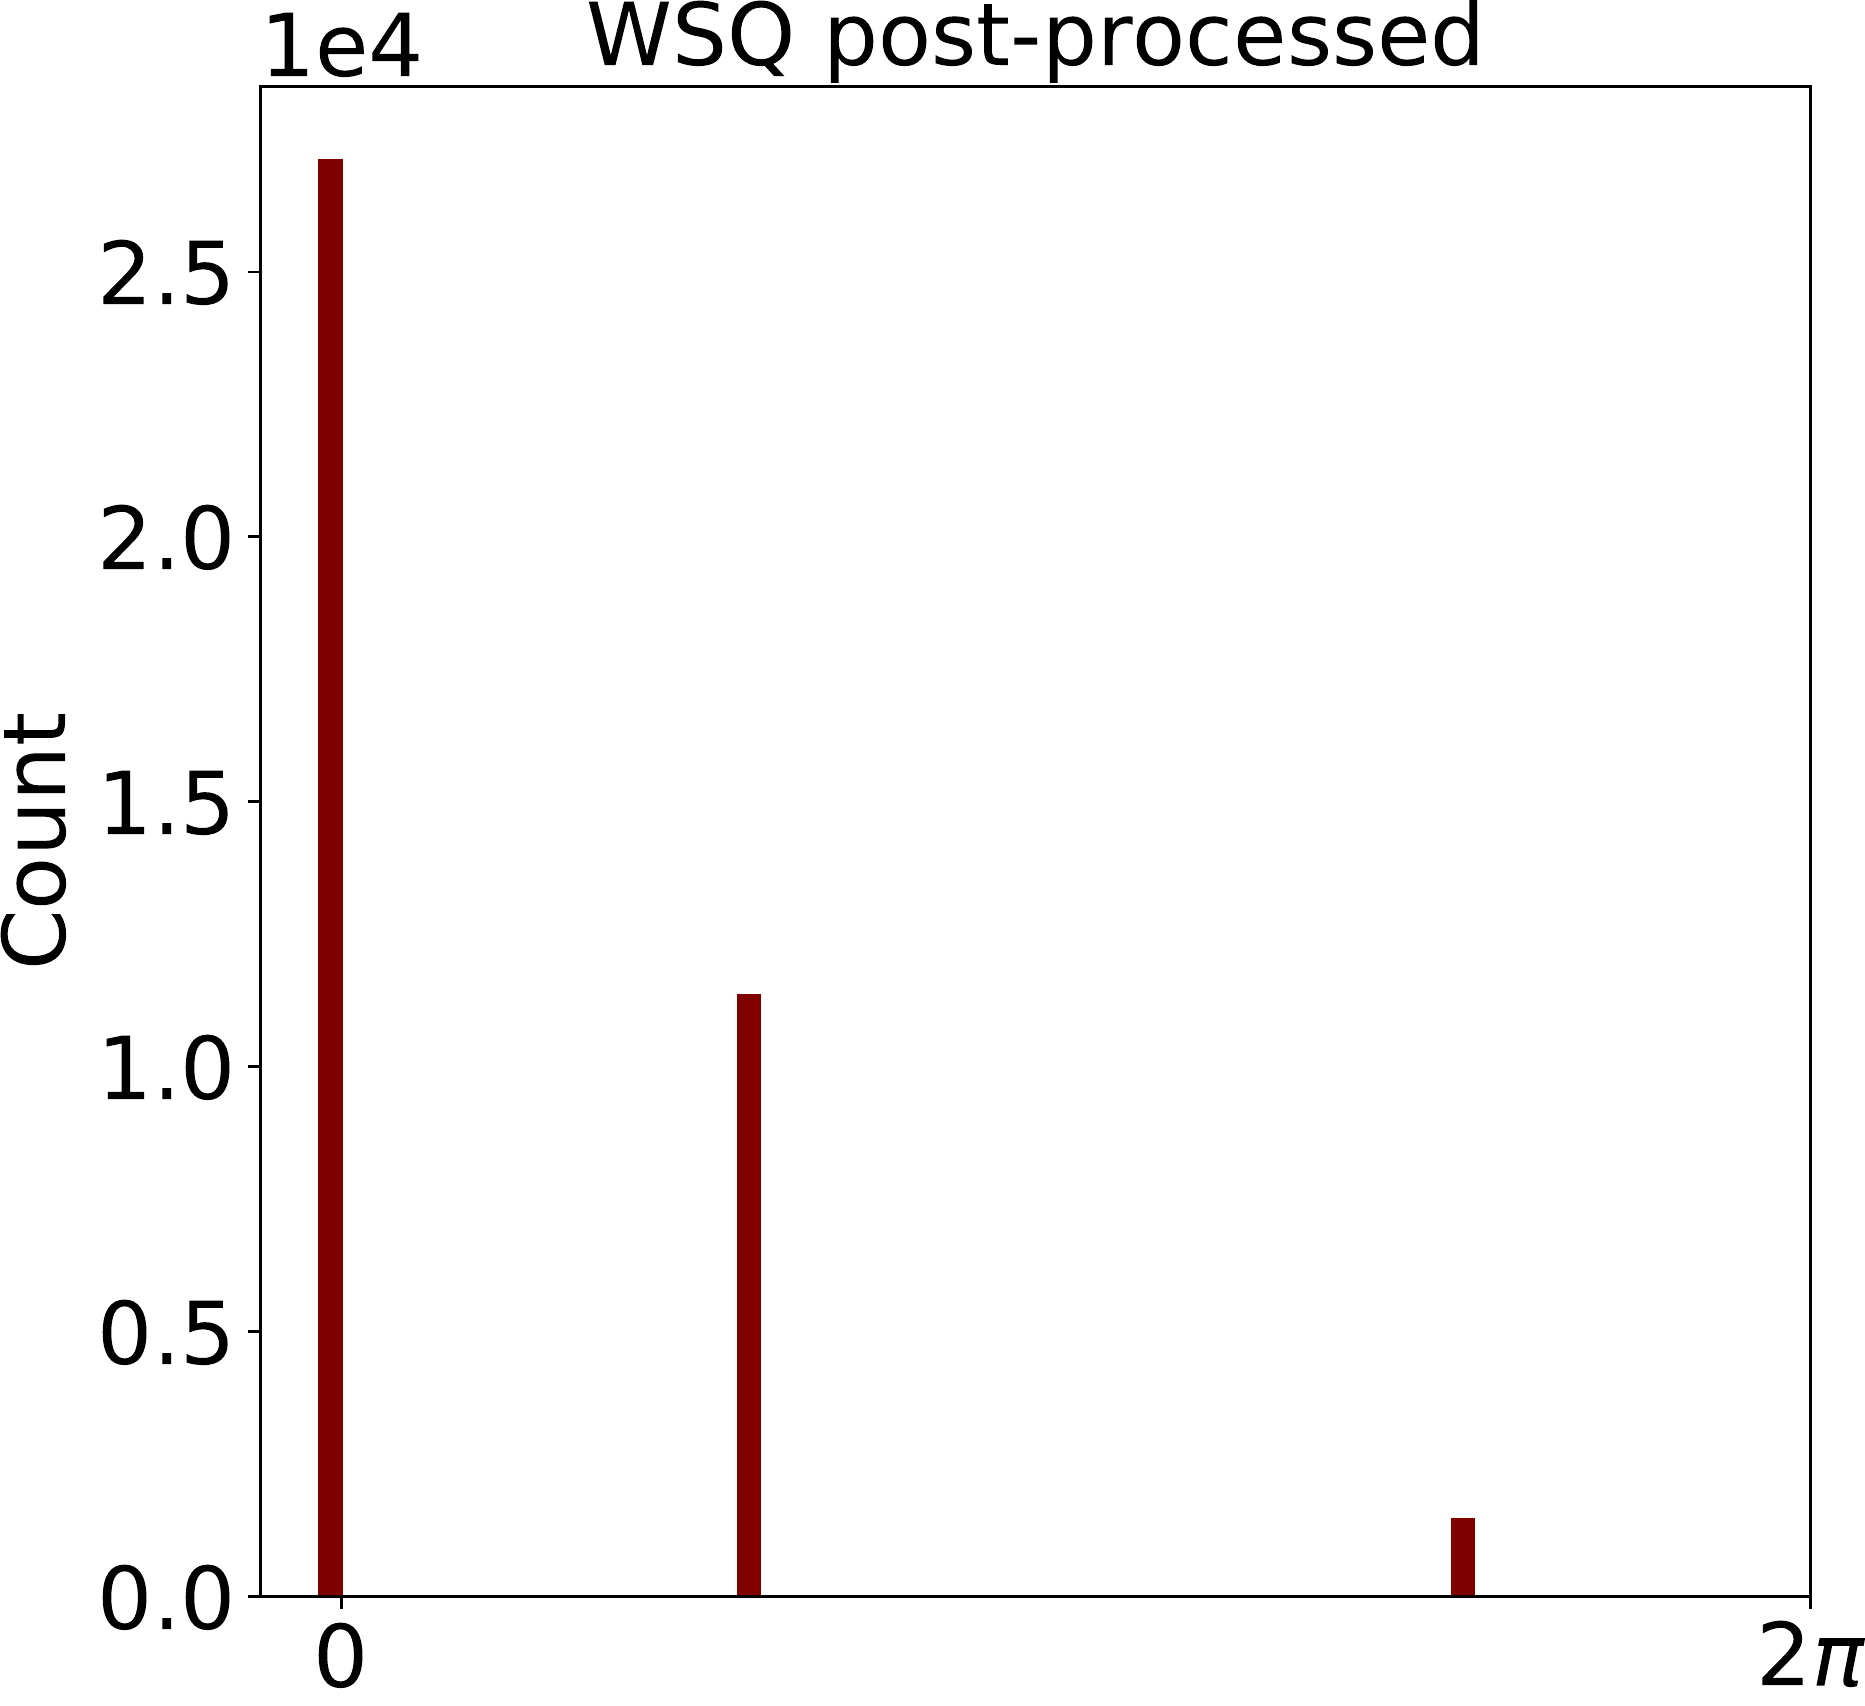}}
        {\includegraphics[width=0.18\linewidth]{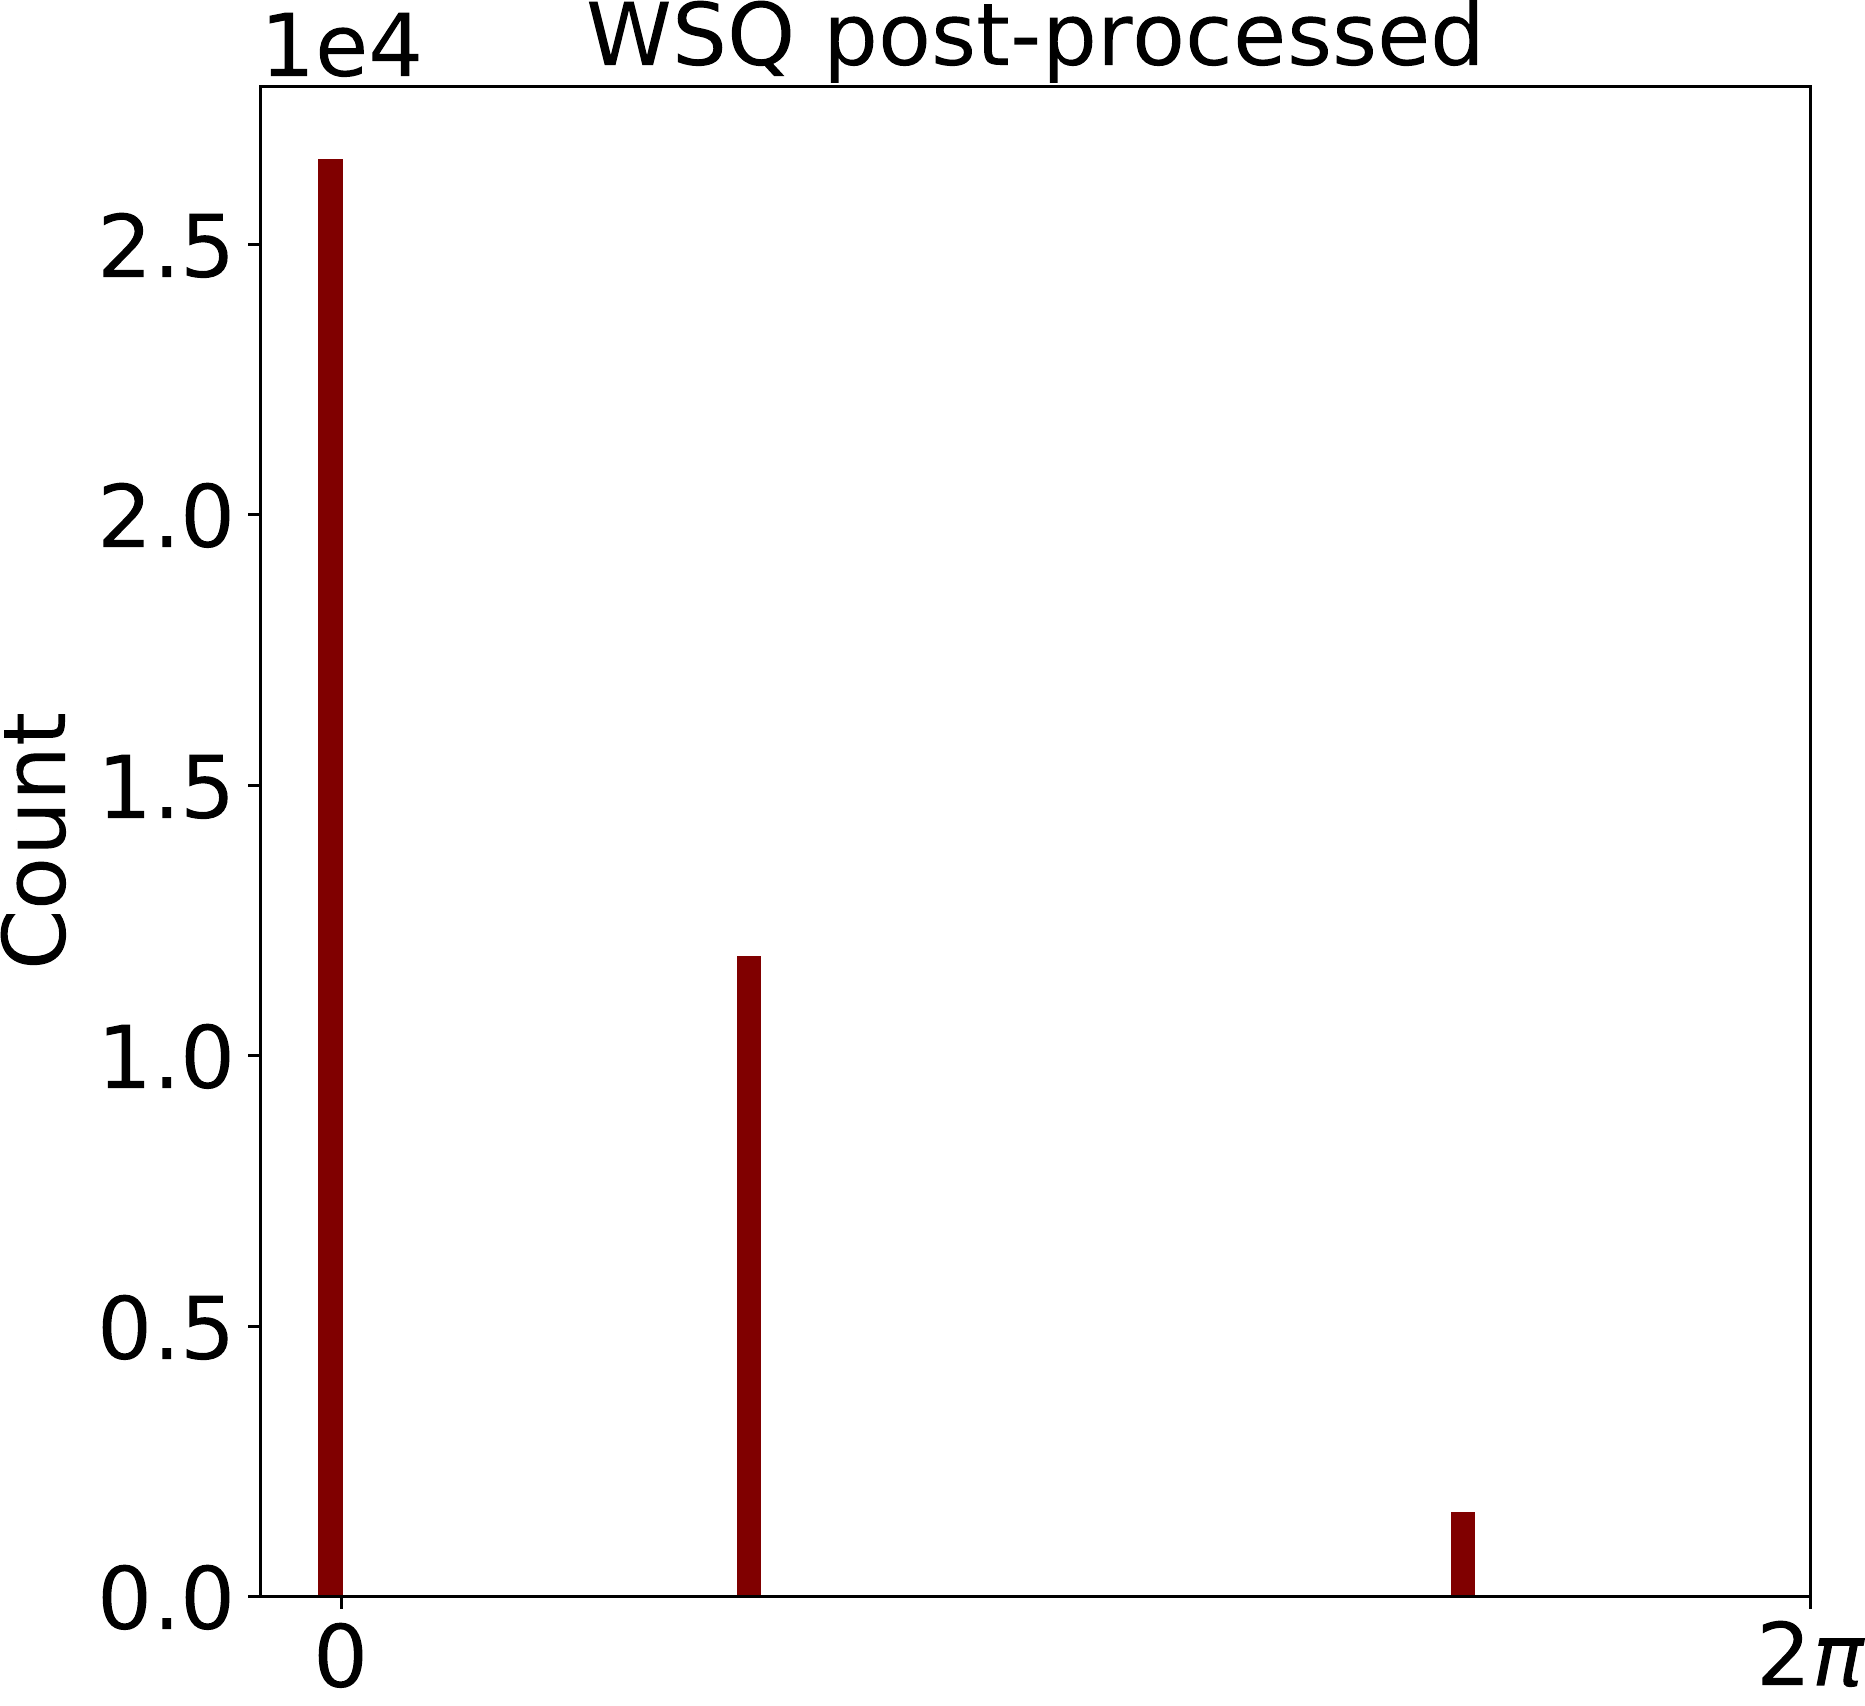}}
        {\includegraphics[width=0.18\linewidth]{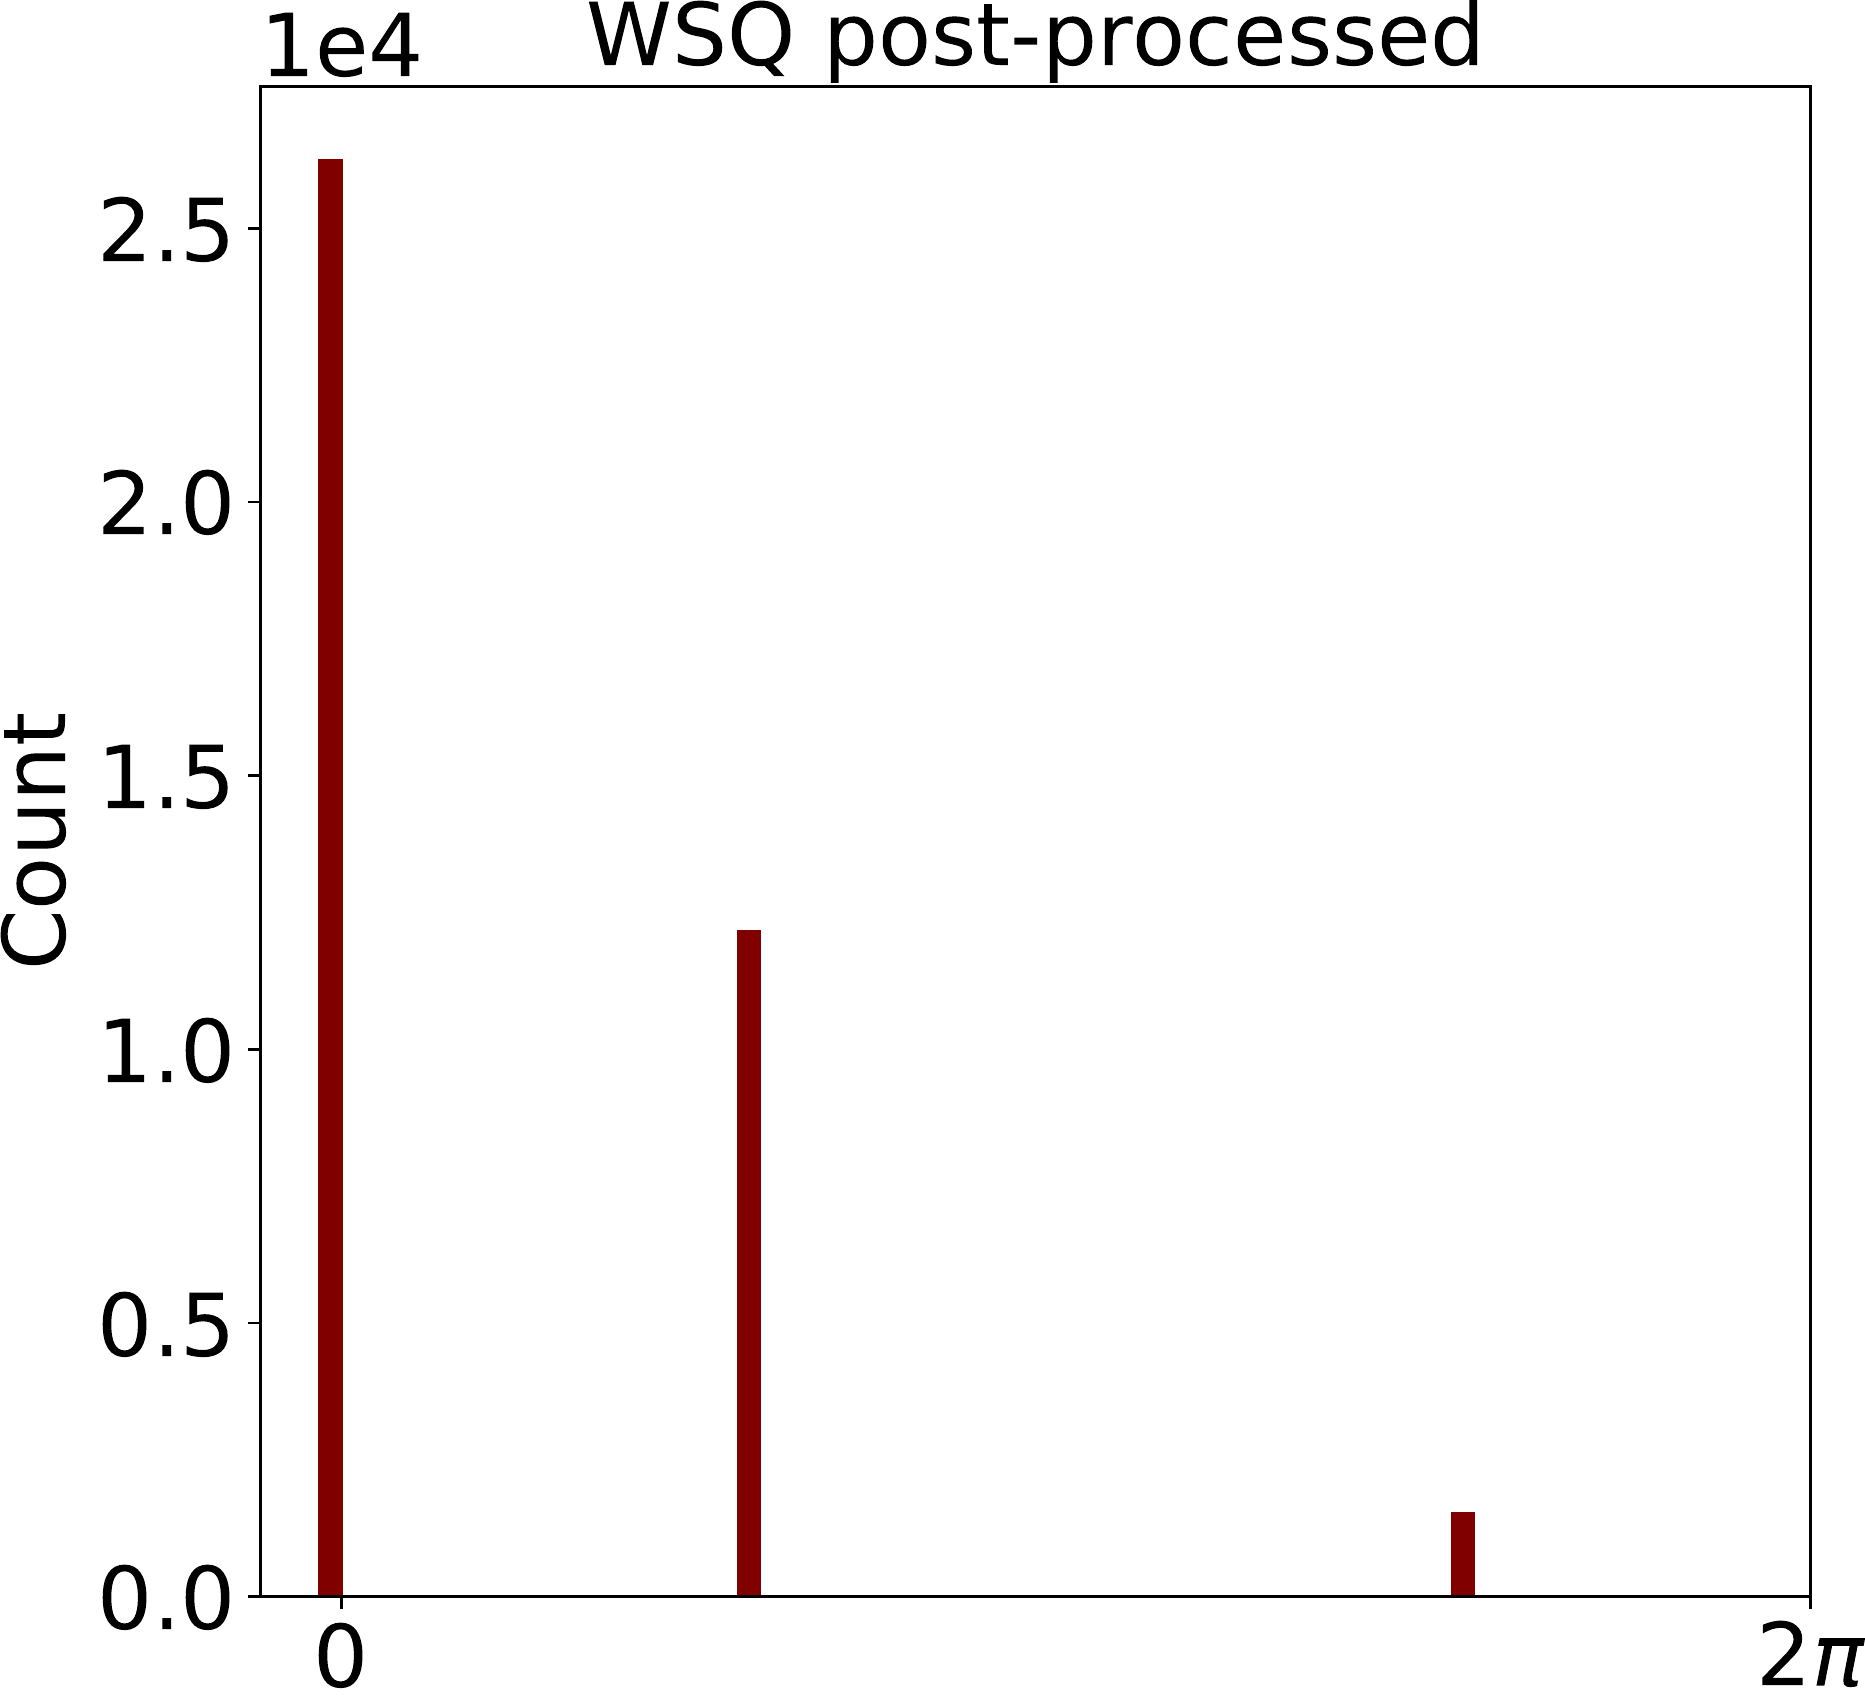}}
        {\includegraphics[width=0.18\linewidth]{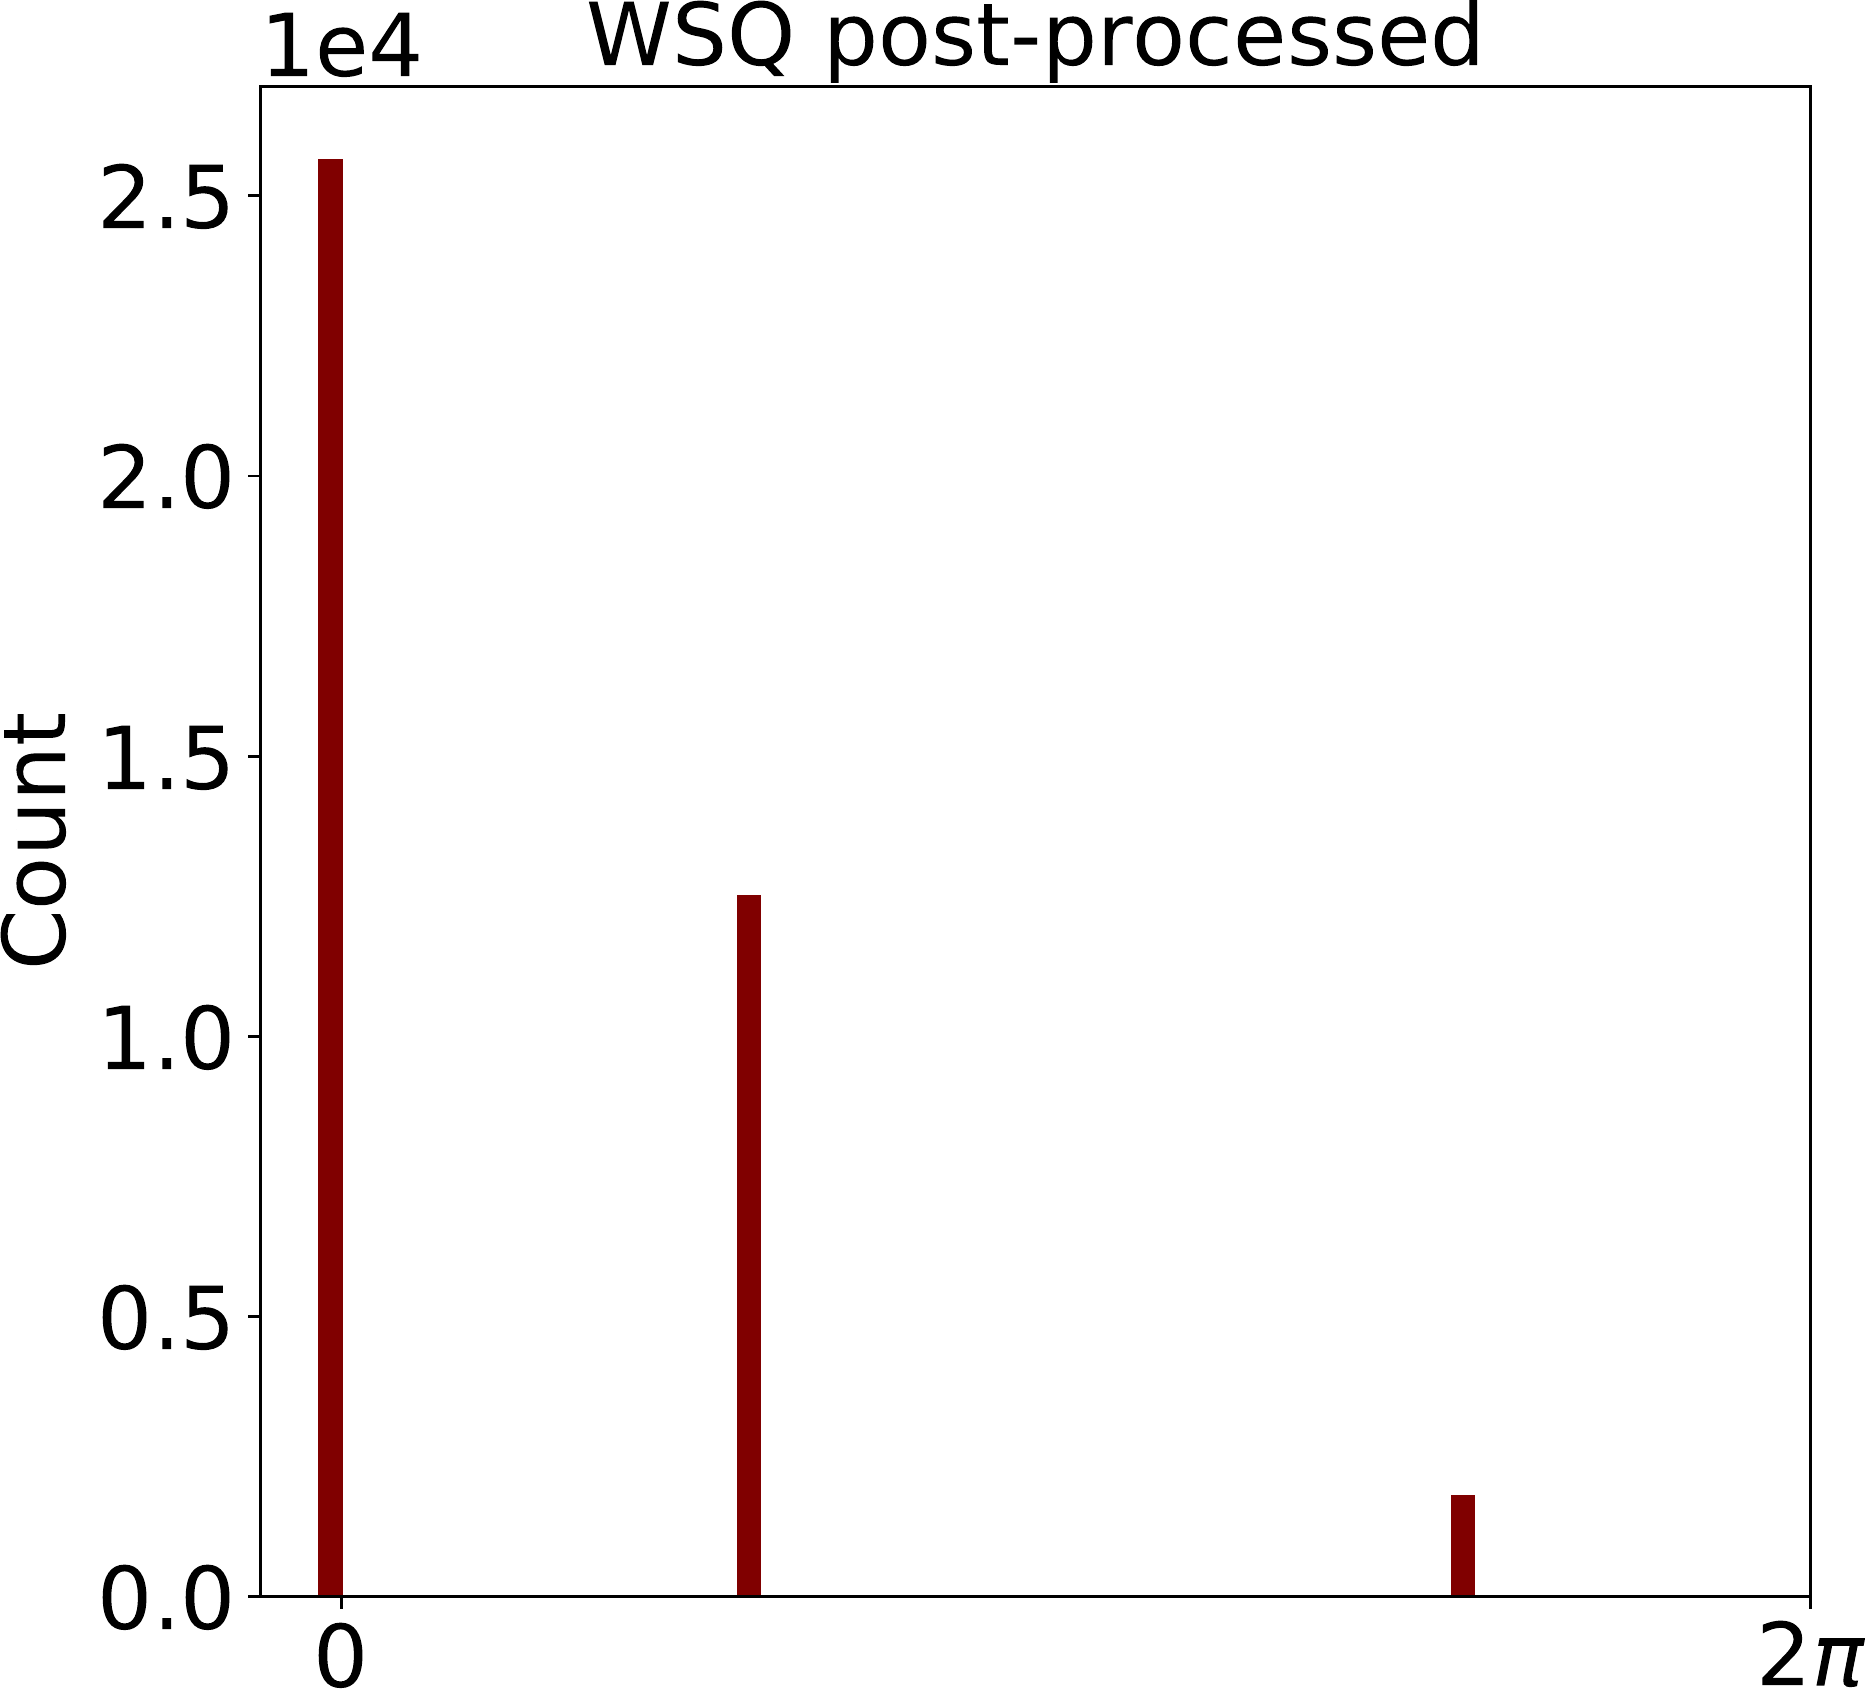}}
        \caption{Weight parameters distribution for layers from first to last in model trained with WSQ after post processing, shown from left to right.}
    \end{subfigure}
    \hfill
    \begin{subfigure}[b]{1\linewidth}
    \centering
        {\includegraphics[width=0.18\linewidth]{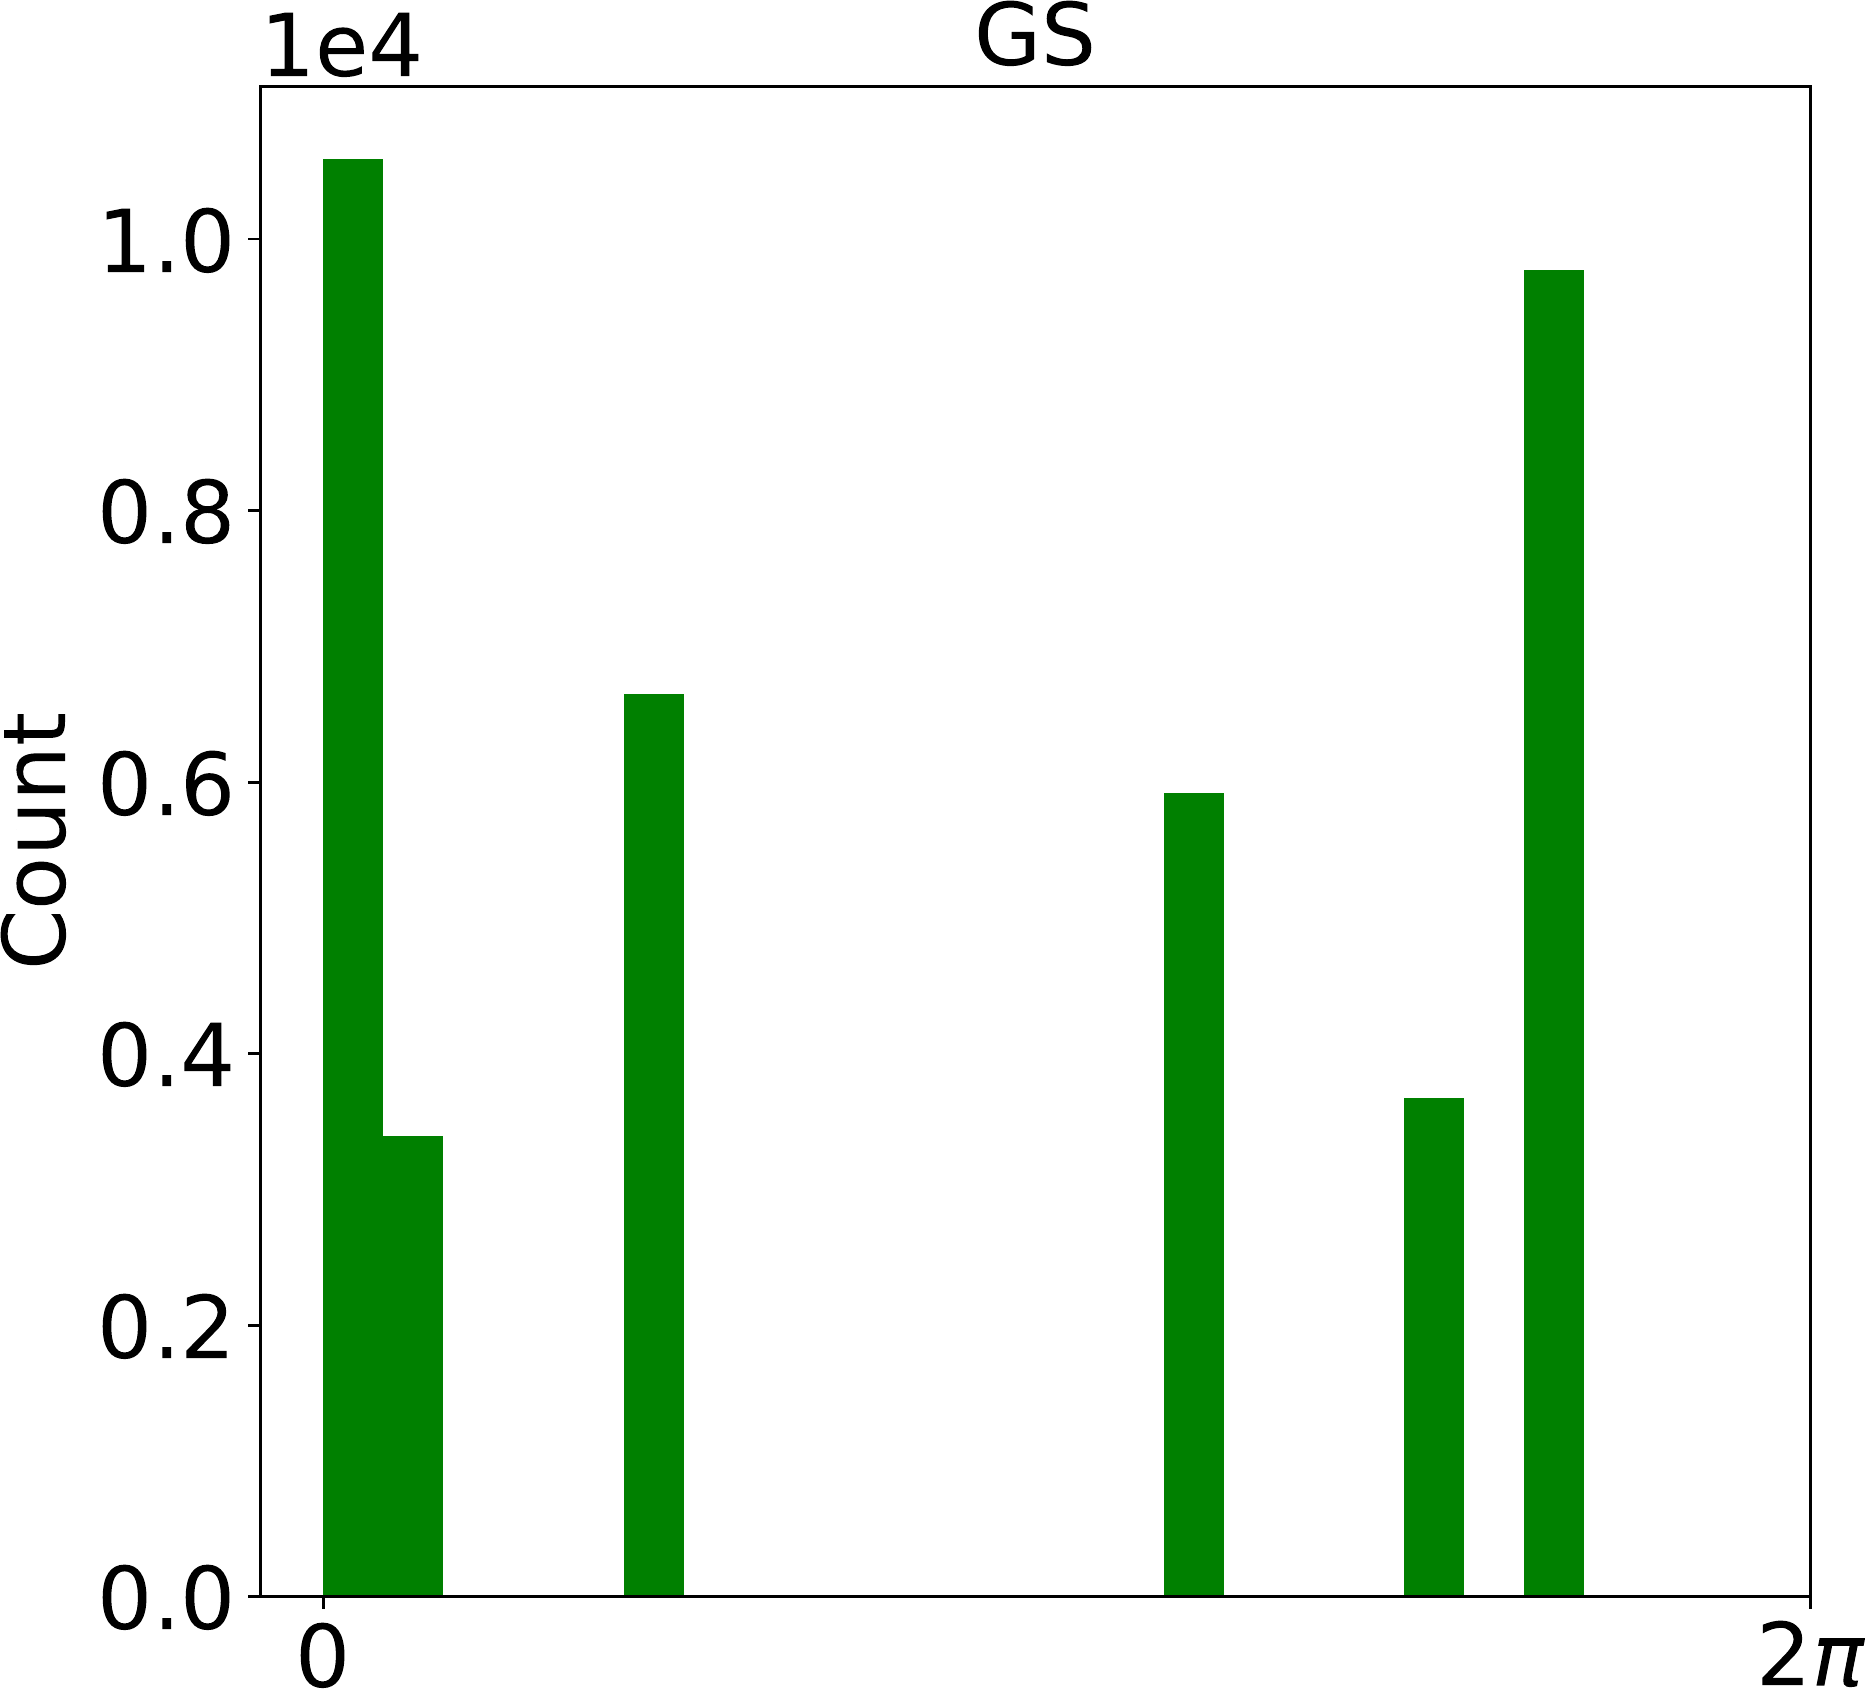}}
        {\includegraphics[width=0.18\linewidth]{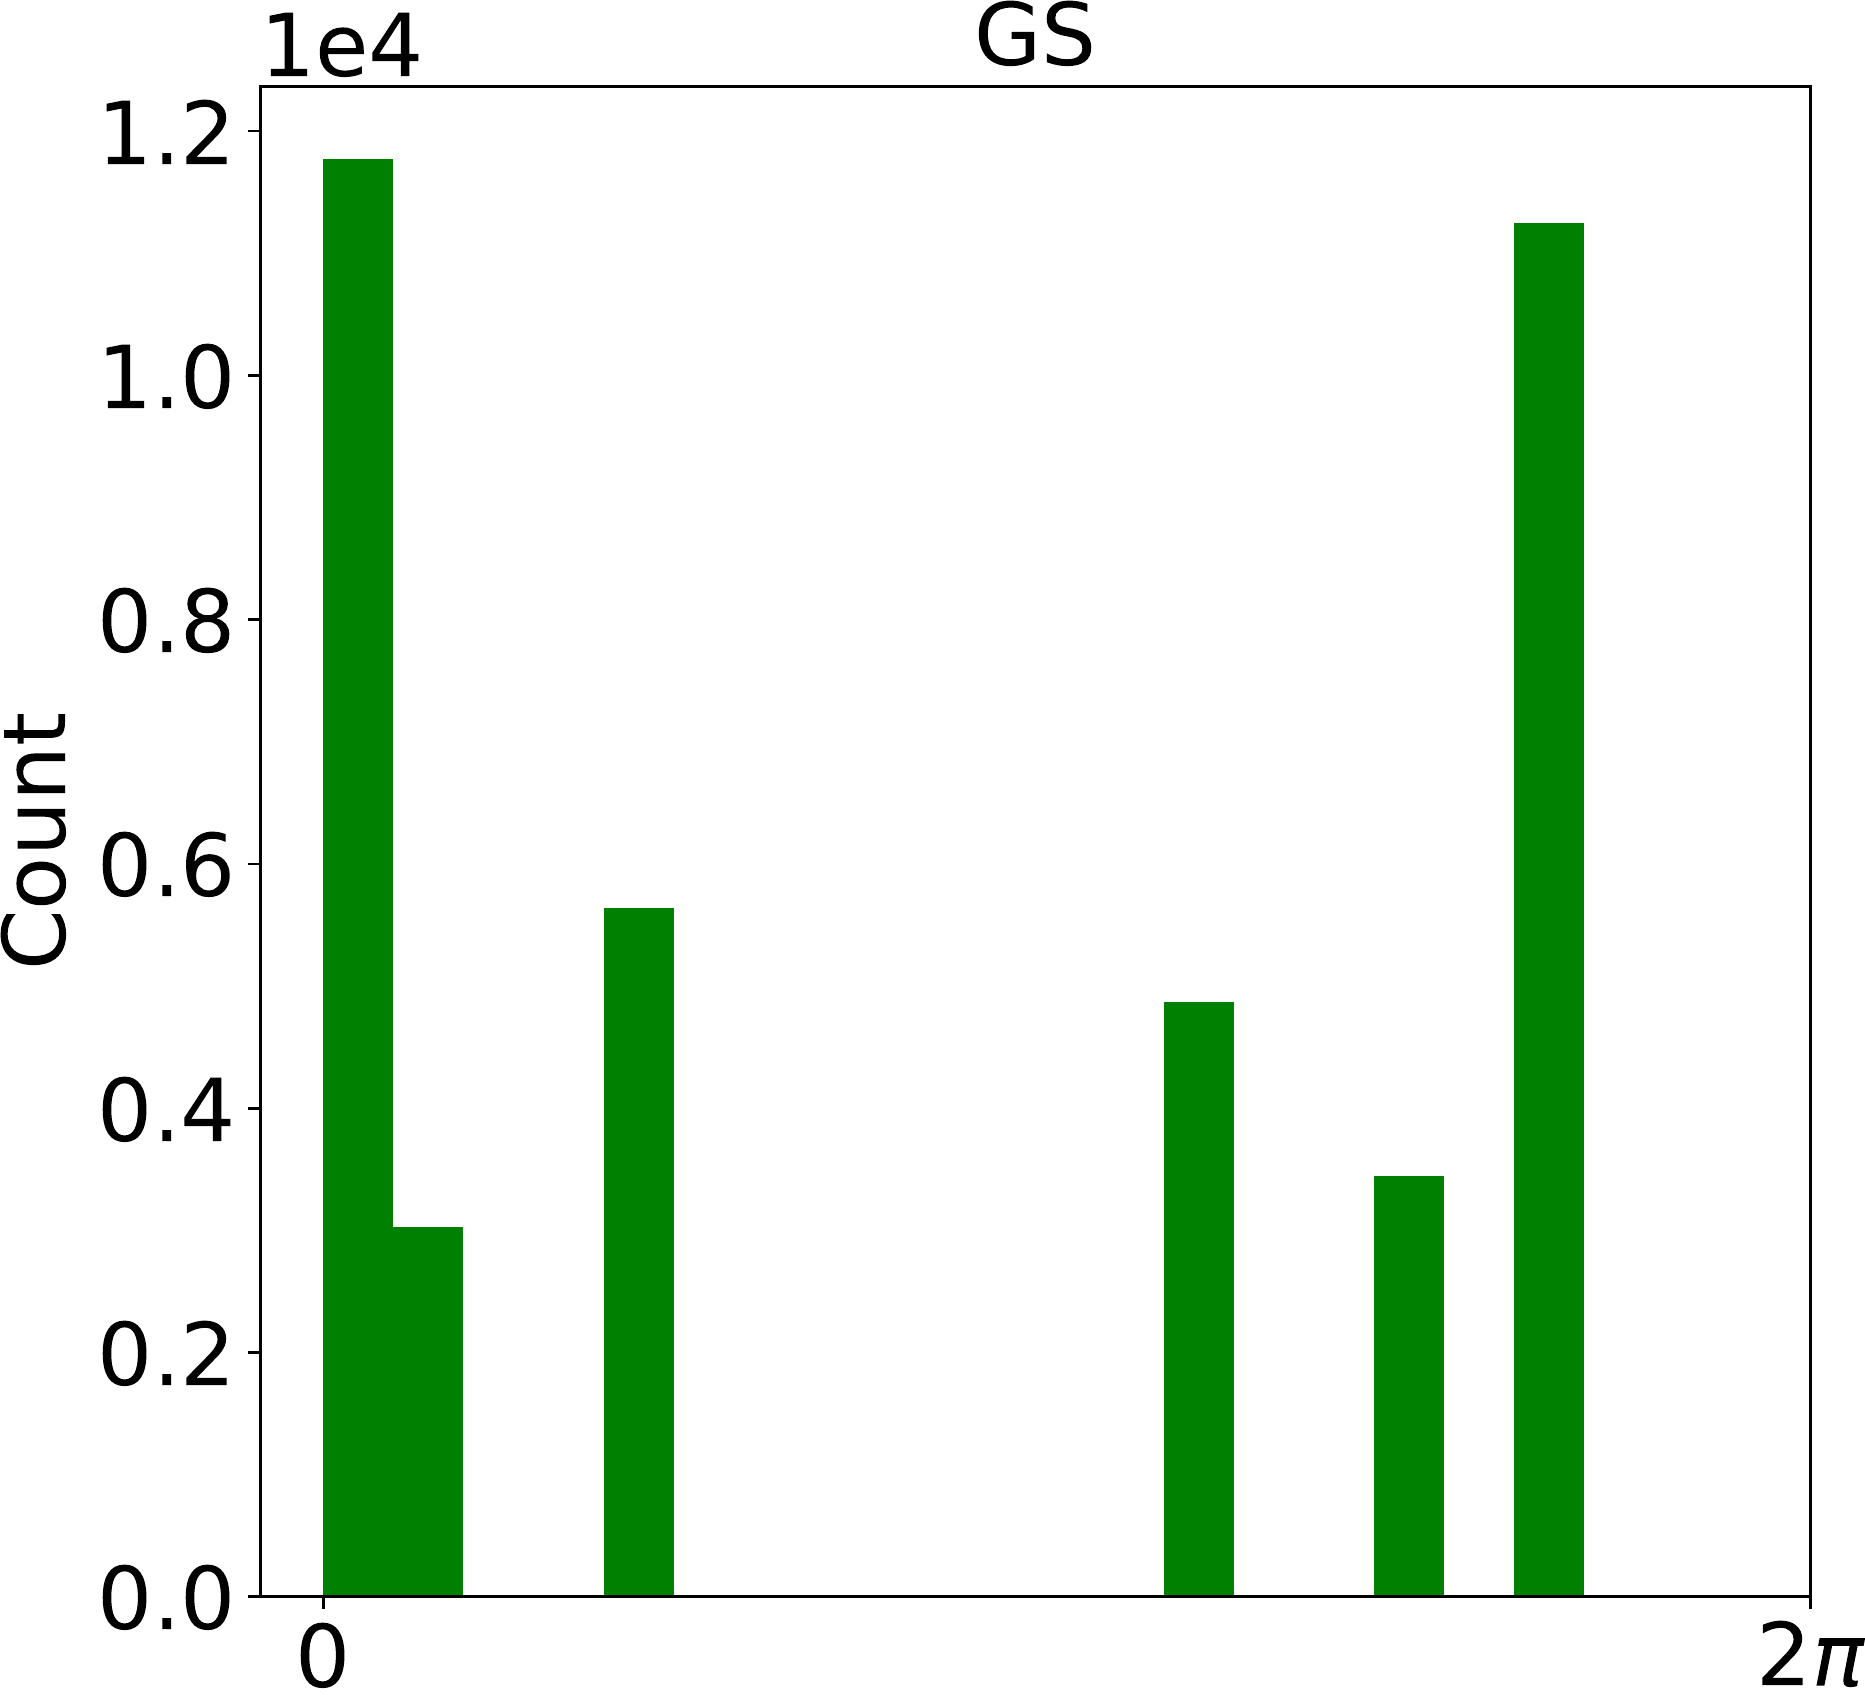}}
        {\includegraphics[width=0.18\linewidth]{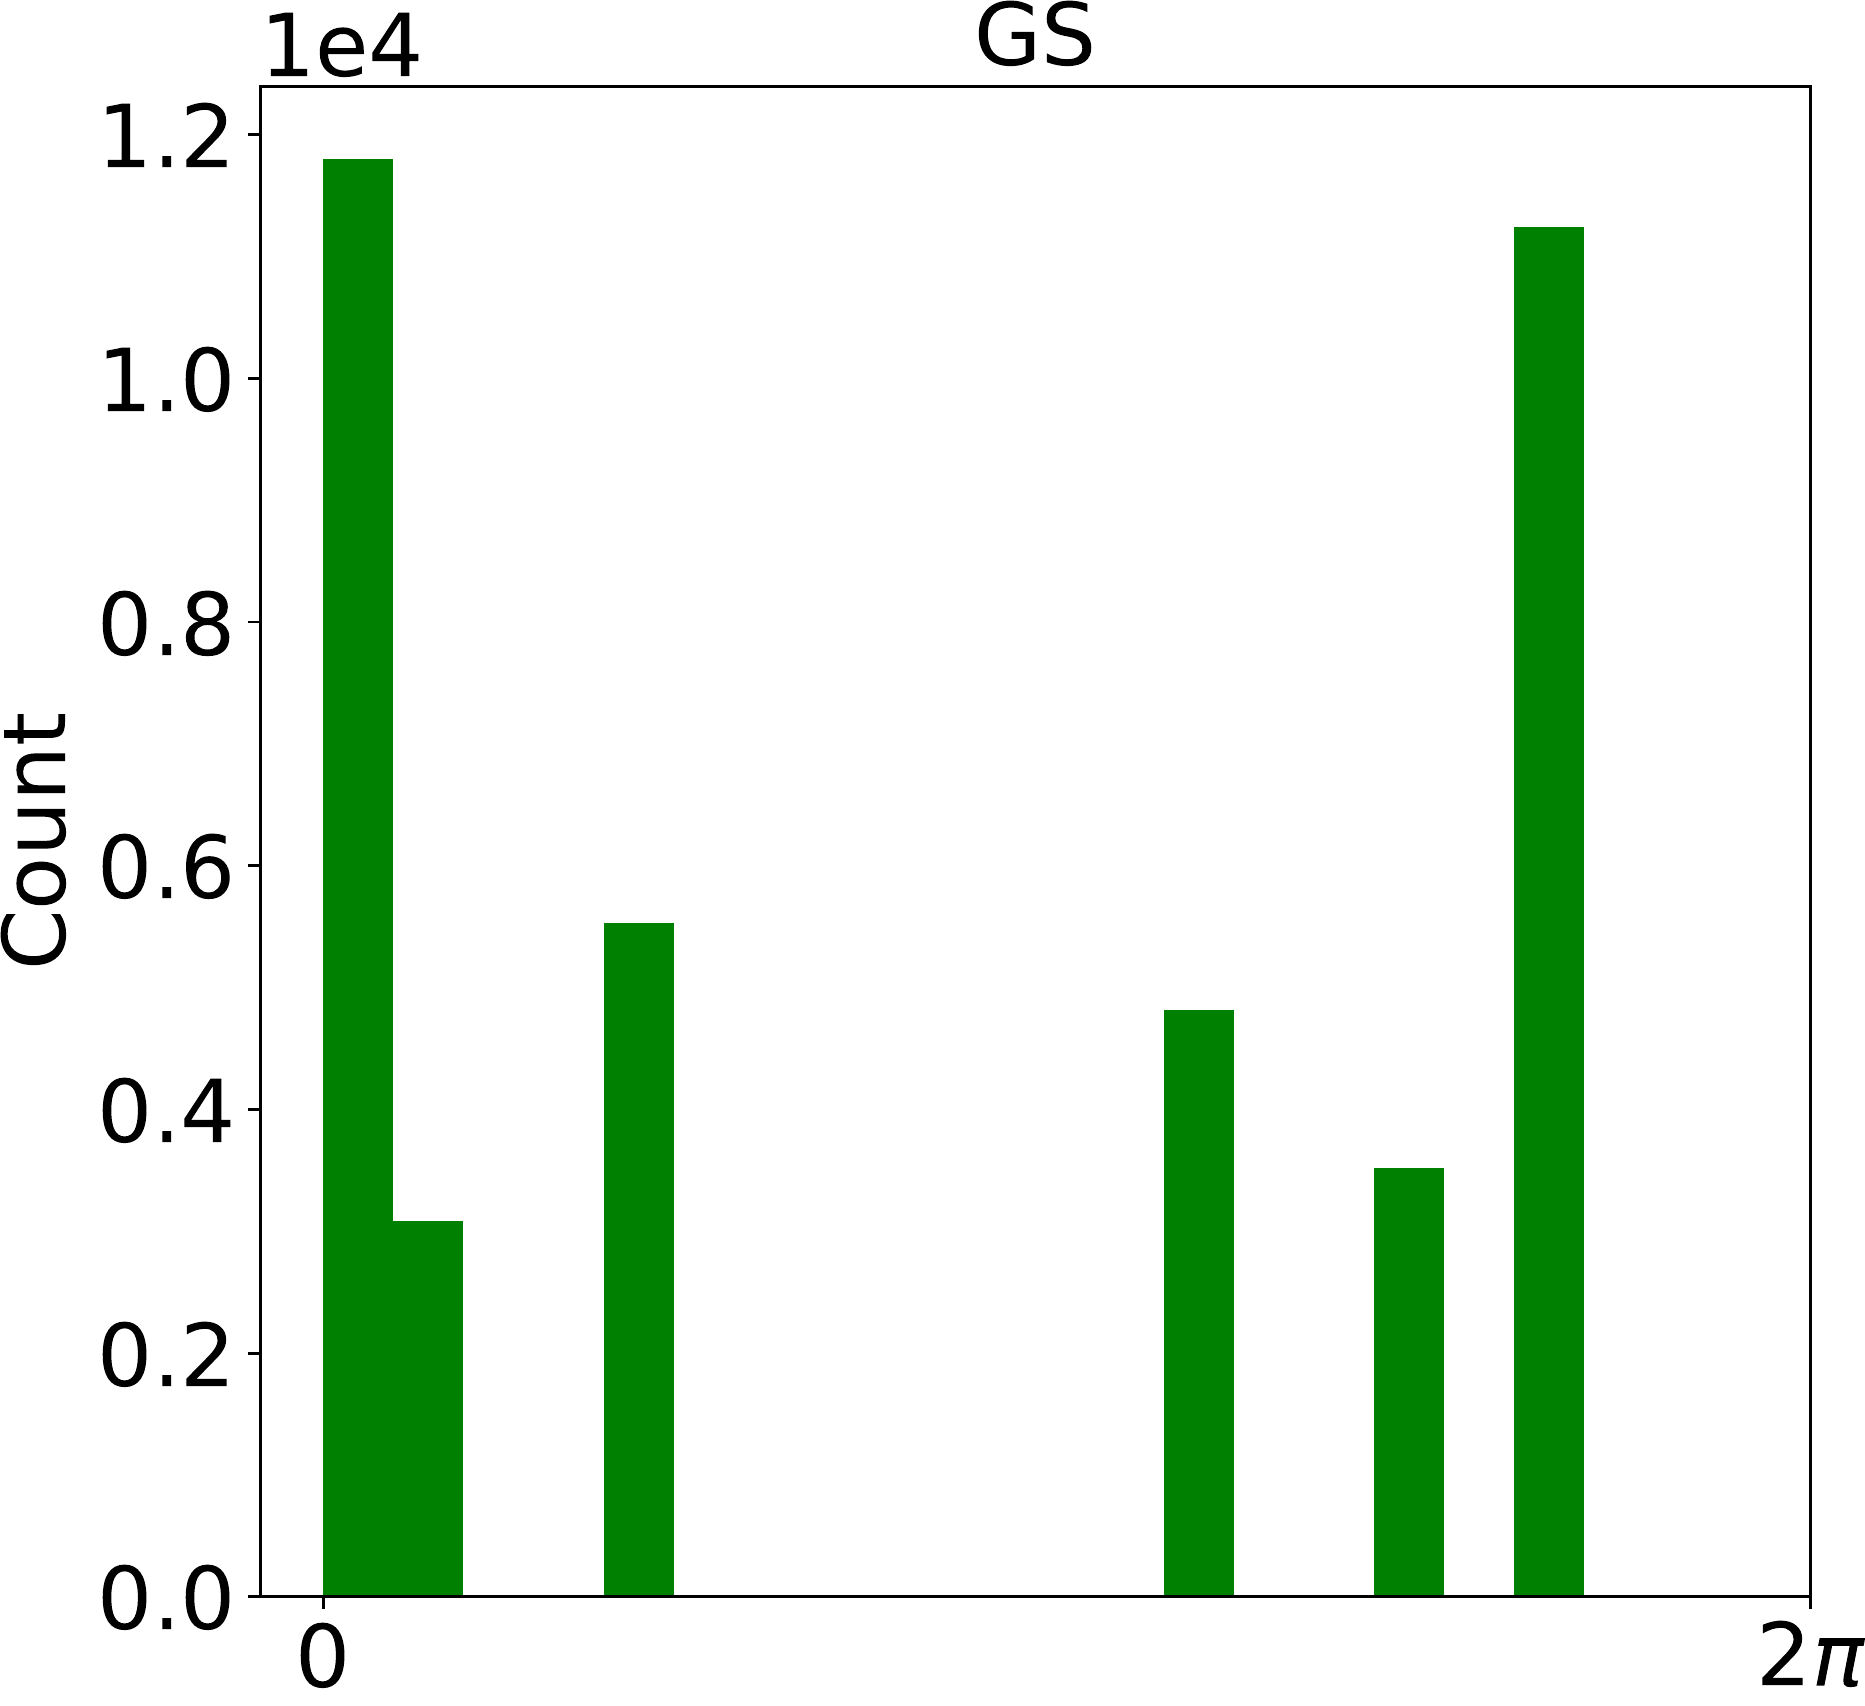}}
        {\includegraphics[width=0.18\linewidth]{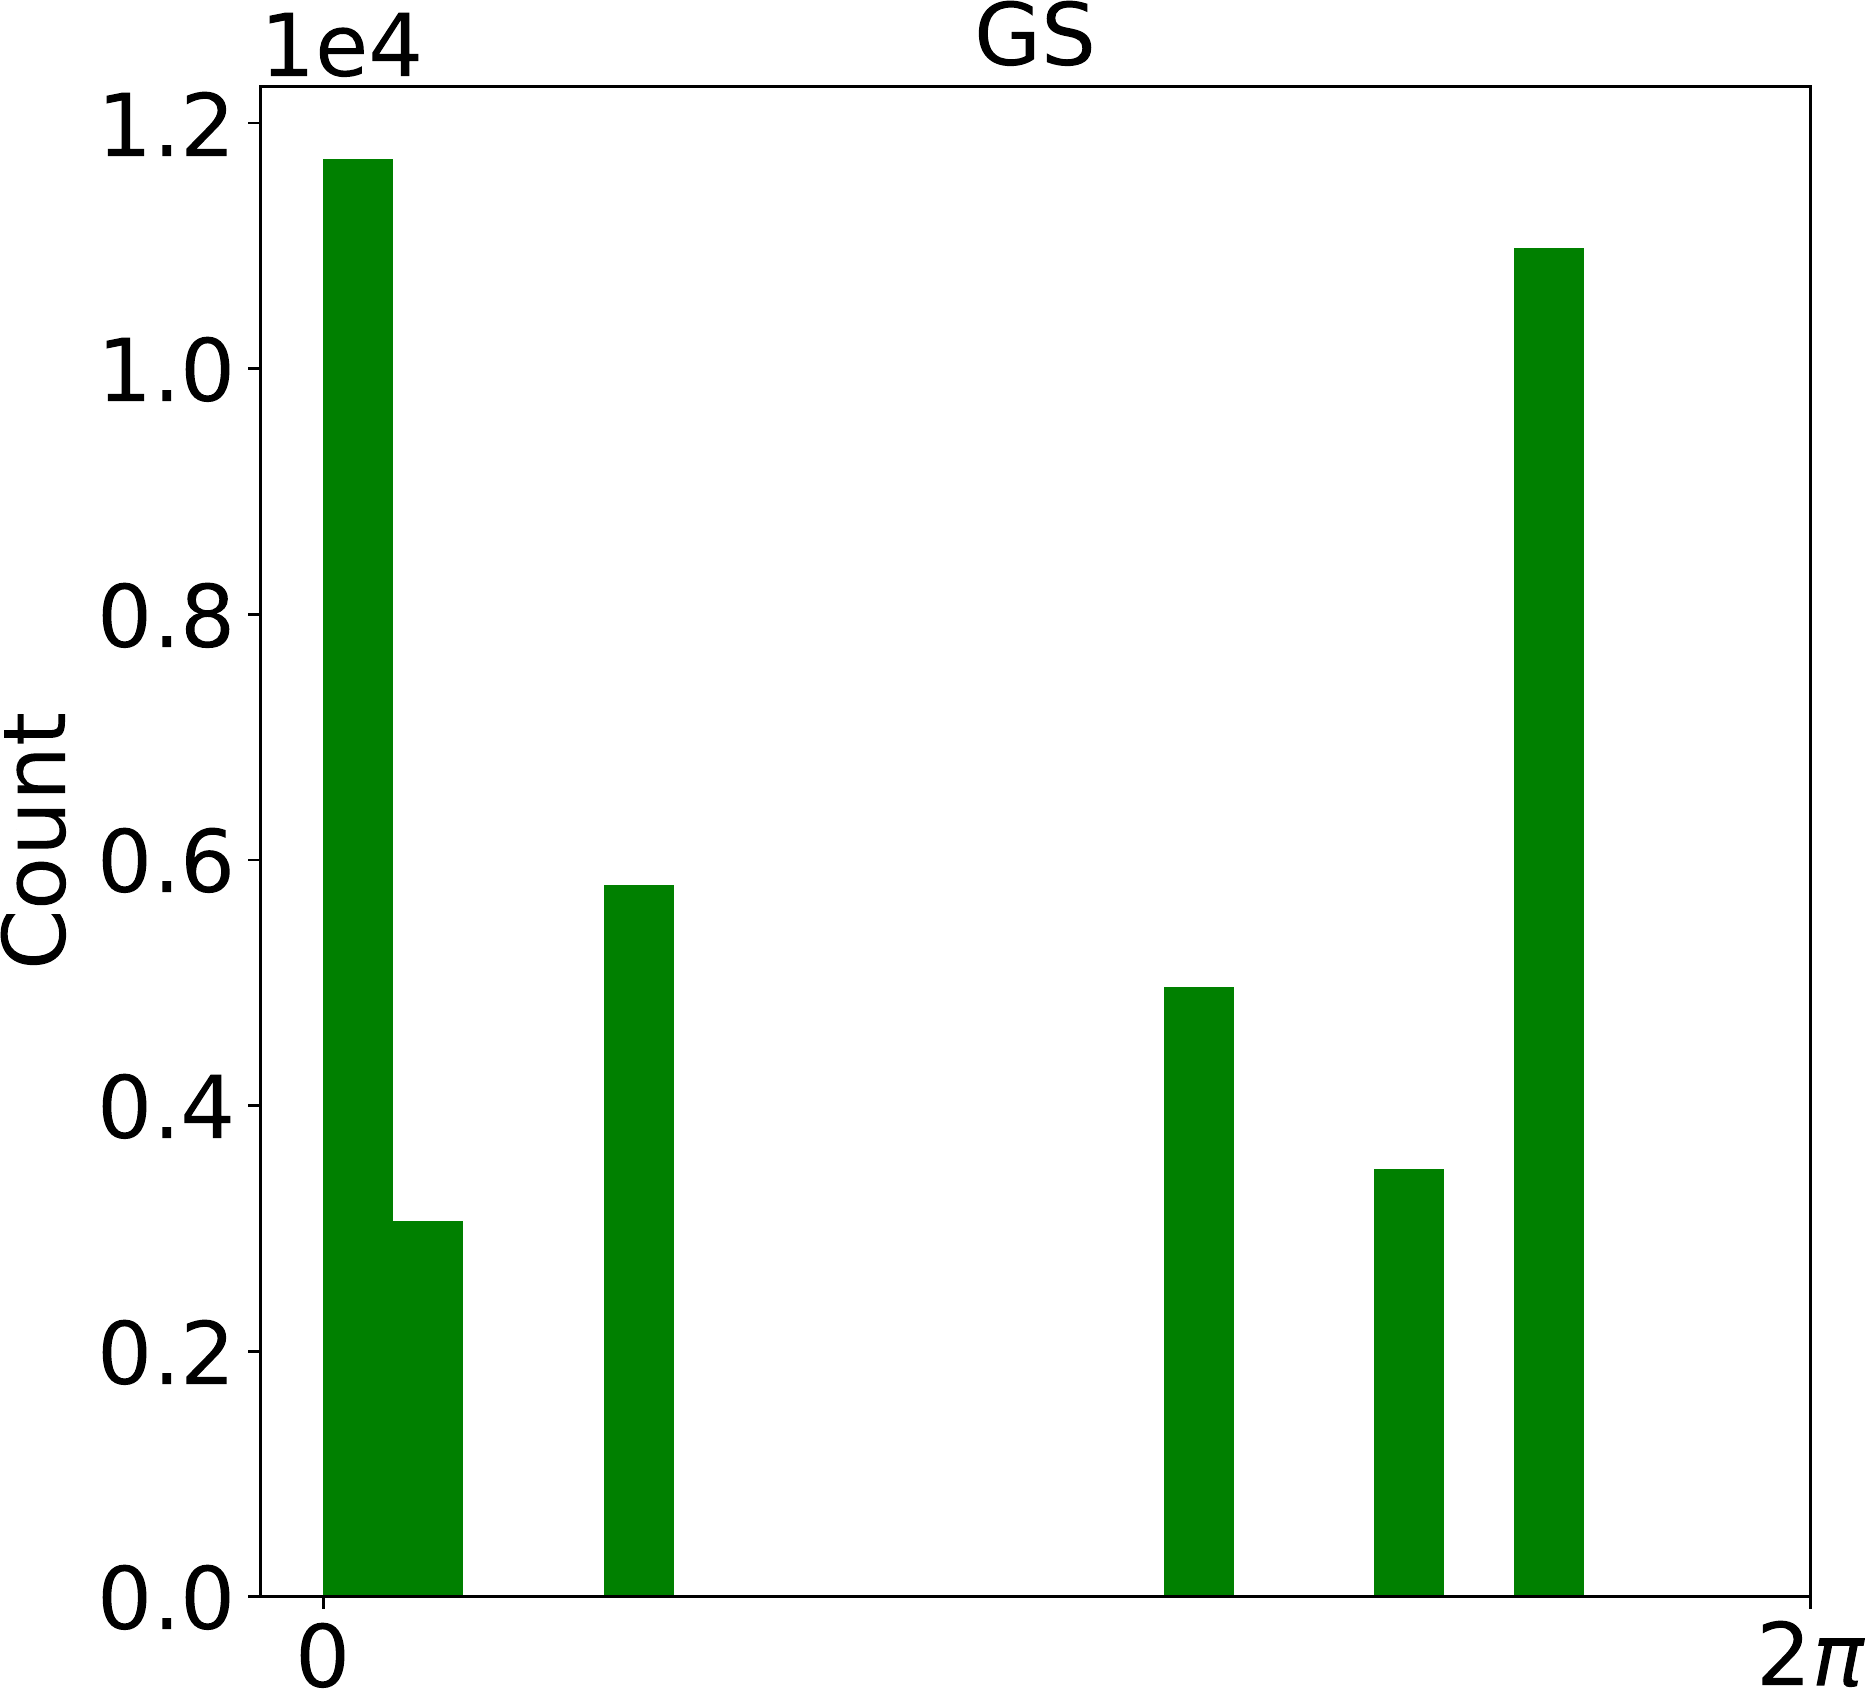}}
        {\includegraphics[width=0.18\linewidth]{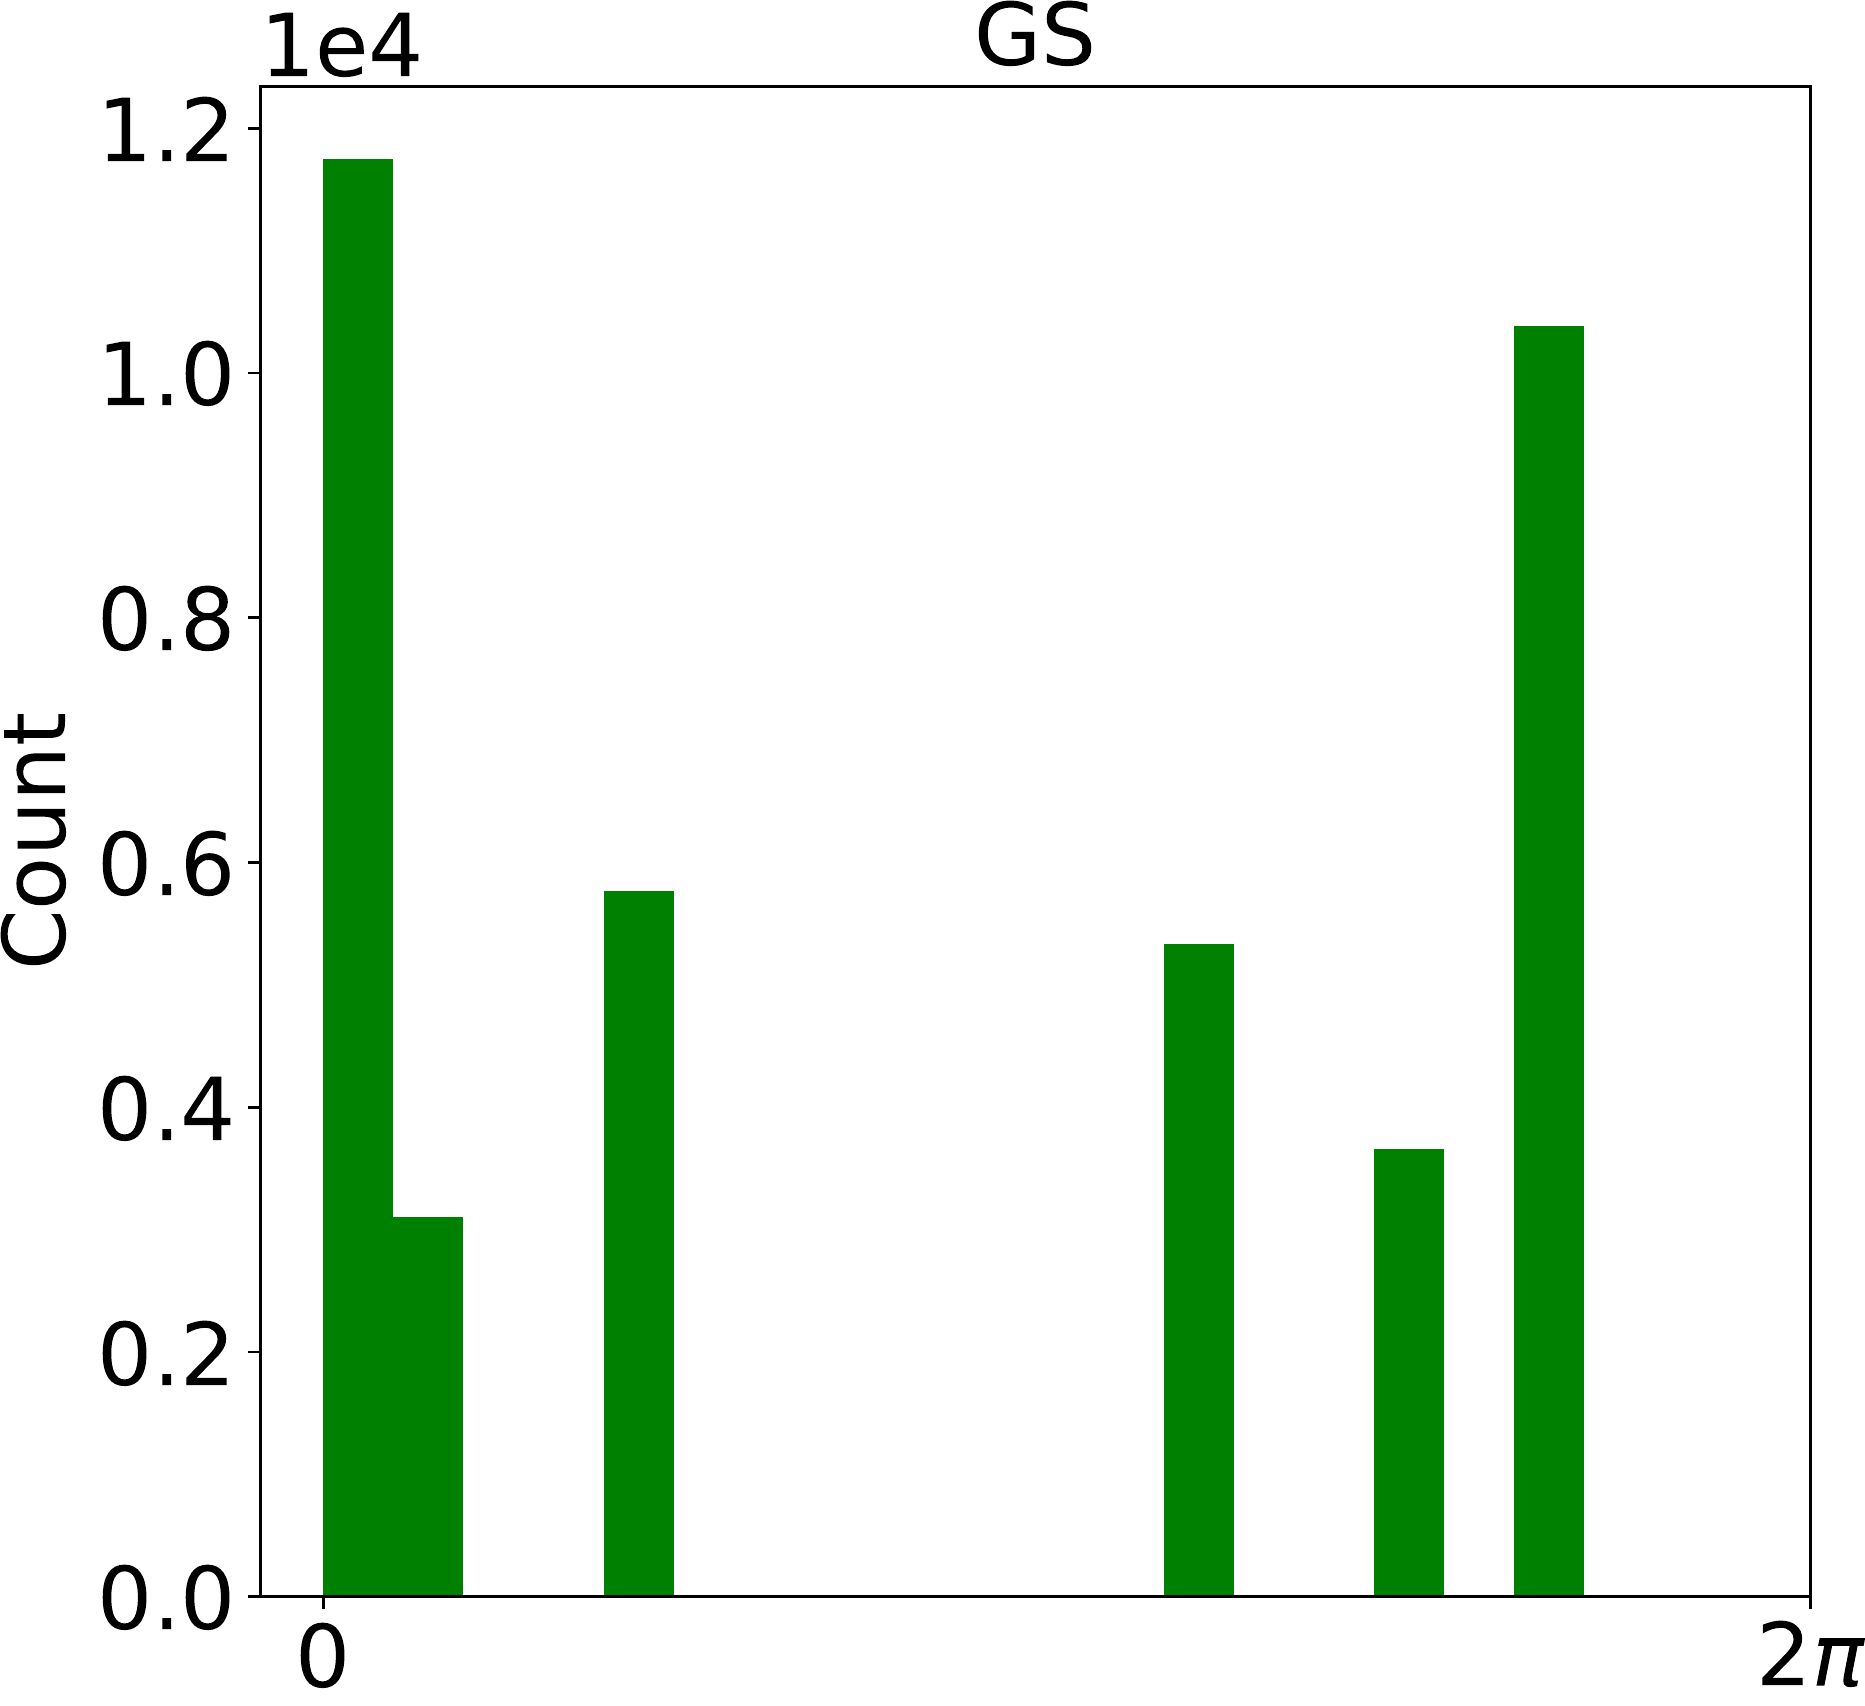}}
        \caption{Weight parameters distribution for layers from first to last in model trained with GS, shown from left to right.}
    \end{subfigure}
    \caption{Weights distribution for each layer in the 5-layer DONN model quantized with full precision, WSQ before and after post processing, and our proposed GS-based framework. }
    \label{fig:weight_ana_each}
\end{figure}

\begin{figure*}[h]
    \centering
    \includegraphics[width=0.7 \linewidth]{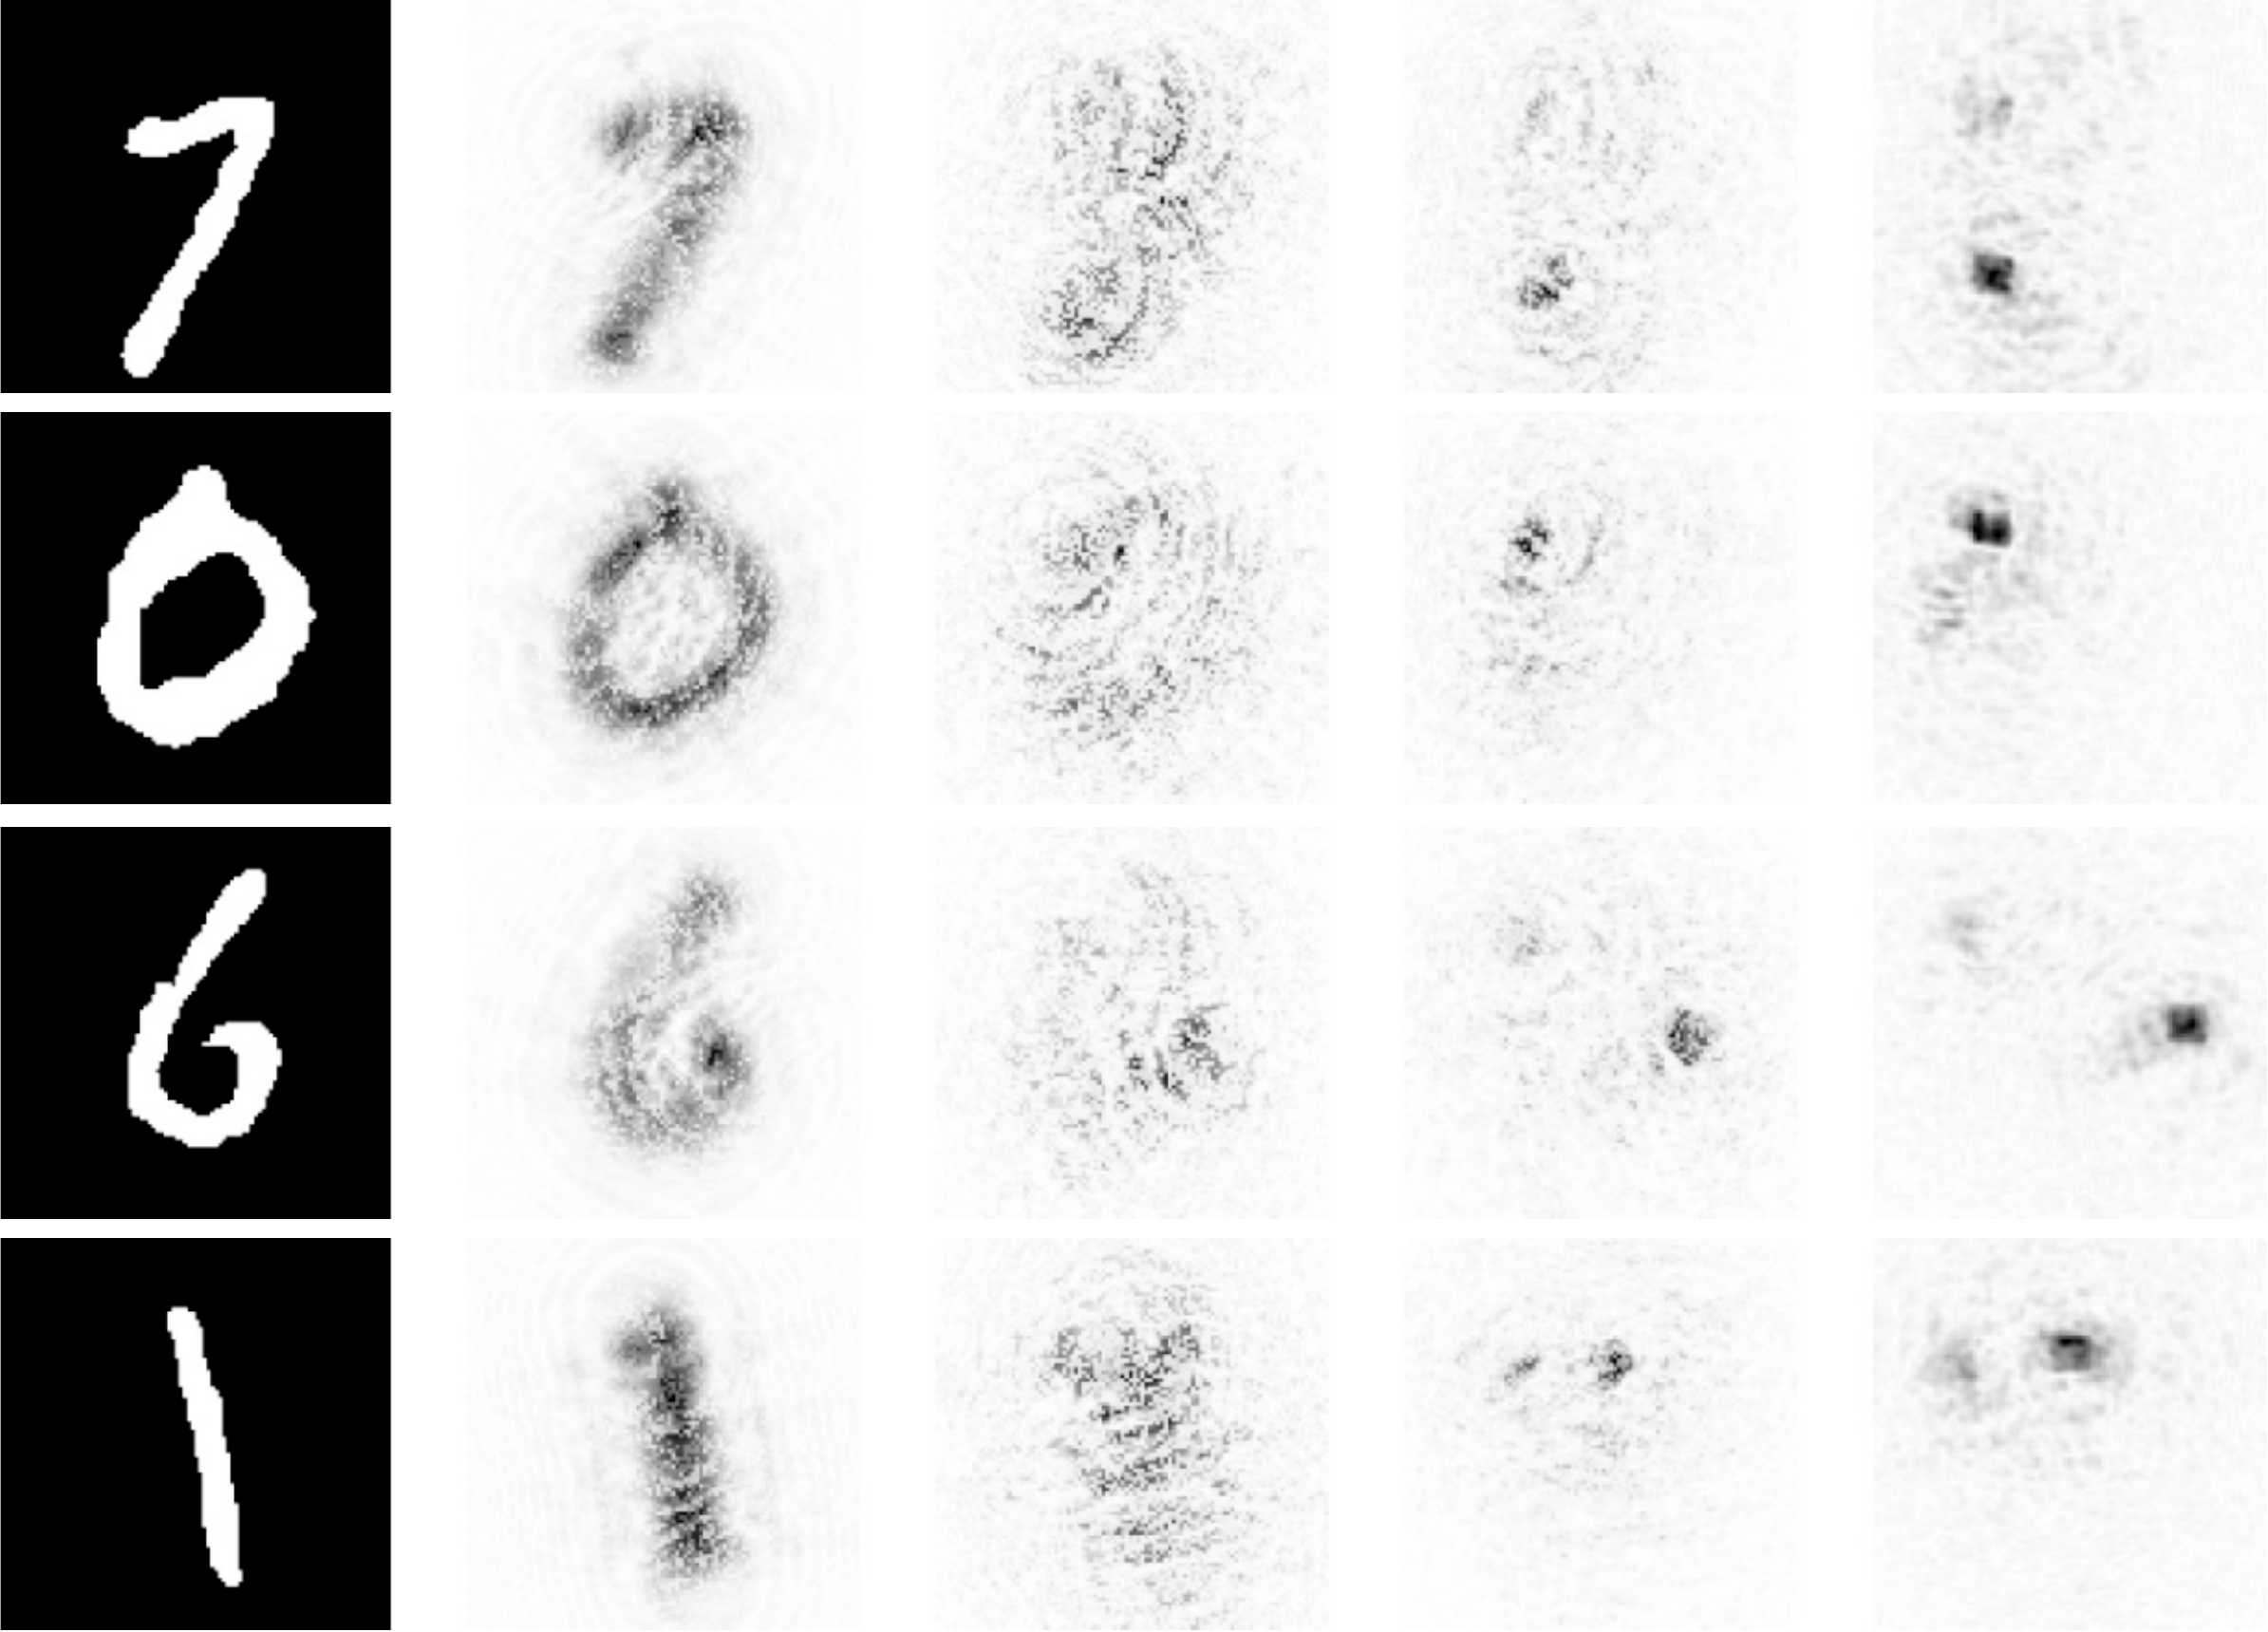}
    \caption{Corresponding propagation simulation of the 3-layer DONN system, in which the simulated intensity distribution precisely matches the experimental measurement shown in Figure \ref{fig:prop_exp}.}
    \vspace{-3mm}
    \label{fig:prop_sim}
\end{figure*}
